# Supplementary material for: Estimation of Conditional Mean Operator under the Bandable Covariance Structure
Source: arXiv:2103.06420 ancillary file (2021-03-11)
Supplement: Supplementary file 1 [file supplementary_material.pdf]

# Supplementary Material of “Estimation of Conditional Mean Operator under the Bandable Covariance Structure”

March 11, 2021

In this supplementary material, we give the proofs of Theorems 2.1-2.2, Lemma 2.3 and Theorems 3.1-3.2 in the main paper, and the proofs of lemmas given in Section A.

## 1 Proof of Theorem 1

In this section, we prove Theorem 2.1. First, we present Lemma 1.1 which is necessary for the proof of Theorem 2.1.

**Lemma 1.1.** *Let  $p$  and  $k$  be positive integers with  $k < p$ . Suppose  $\Sigma \in \mathcal{C}_p$  is a  $k$ -band matrix, and let  $\Sigma^{-1} = (w_{ij})$ . For all  $a > 0$  and all sufficiently large  $k$  with  $p > k \vee (ak \log k)$ ,*

$$\max_j \sum_i \{|w_{ij}| : |i - j| > ak \log k\} \leq -\frac{2C}{\log q} k^{2a \log q + 1},$$

where  $q = (\kappa^{1/2} - 1)/(\kappa^{1/2} + 1)$ ,  $C = \{\|\Sigma^{-1}\| \vee (1 + \kappa^{1/2})^2\}/(2\|\Sigma\|)$ , and  $\kappa$  is the spectral condition number of  $\Sigma$ .

*Proof.* Since  $\Sigma$  is a  $k$ -band matrix,

$$|w_{ij}| \leq Cq^{2|i-j|/k}, \quad i, j \in \{1, 2, \dots, p\},$$

where  $q = (\kappa^{1/2} - 1)/(\kappa^{1/2} + 1)$ ,  $C = \{||\Sigma^{-1}|| \vee (1 + \kappa^{1/2})^2\}/(2||\Sigma||)$  and  $\kappa$  is the spectral condition number of  $\Sigma$  defined as  $\lambda_{\max}(\Sigma)/\lambda_{\min}(\Sigma)$  (Demko et al., 1984, Theorem 2.4). Note that

$$\begin{aligned} \max_j \sum_{\{i: |i-j| > ak \log k\}} q^{2|i-j|/k} &\leq \frac{2}{1 - q^{2/k}} q^{2a \log k} \\ &= \frac{2}{k(1 - q^{2/k})} k^{\log q^{2a+1}}, \end{aligned}$$

and

$$\lim_{k \rightarrow \infty} k(q^{2/k} - 1) = \left( \frac{dq^{2x}}{dx} \right)_{x=0} = 2 \log q.$$

Thus, we get

$$\max_j \sum_{\{i: |i-j| > ak \log k\}} q^{2|i-j|/k} \leq \frac{2}{-\log q} k^{\log q^{2a+1}}$$

for all sufficiently large  $k$ . □

Now we prove Theorem 2.1.

*Proof of Theorem 2.1.* Let  $B_k(\Sigma_0)^{-1} = (w_{ij}^*)$ . We have

$$\begin{aligned} \sum_{i \in I_j} |w_{ij}| &\leq \sum_{i \in I_j} |w_{ij}^*| + \sum_{i \in I_j} |w_{ij} - w_{ij}^*| \\ &\leq \sum_{i \in I_j} |w_{ij}^*| + ||\Sigma_0^{-1} - B_k(\Sigma_0)^{-1}||_1, \end{aligned}$$

where  $I_j = \{i \in \{1, 2, \dots, p\} : |i - j| > ak \log k\}$ . By Lemma A.1, there exists some positive constant  $C_1$  depending only on  $M$ ,  $M_0$  and  $M_1$  such that

$$||\Sigma_0^{-1} - B_k(\Sigma_0)^{-1}||_1 \leq C_1 k^{-\alpha}, \quad (1)$$

for all sufficiently large  $k$ .

For the upper bound of  $\sum_{i \in I_j} |w_{ij}^*|$ , Lemma 1.1 gives that, for all sufficiently large  $k$  with  $p > k \vee (ak \log k)$ ,

$$\max_j \sum_i \{|w_{ij}^*| : |i - j| > ak \log k\} \leq -\frac{2C_2}{\log q} k^{2a \log q + 1}, \quad (2)$$

where  $q = (\kappa^{1/2} - 1)/(\kappa^{1/2} + 1)$ ,  $C_2 = \{\|\Sigma^{-1}\| \vee (1 + \kappa^{1/2})^2\}/(2\|\Sigma\|)$  and  $\kappa$  is the spectral condition number of  $\Sigma$ . By collecting the inequalities (1) and (2), we complete the proof.  $\square$

## 2 Proof of Theorem 2

In this section, we prove Theorem 2.2 which gives the convergence rate of the tapering estimator. First, we present Lemma 2.1 necessary for the proof of Theorem 2.2.

**Lemma 2.1.** *Let  $\Sigma$  and  $\Sigma_0$  be  $p \times p$ -symmetric matrices and  $\Sigma^{(\epsilon_n)} = \Sigma + [\{\epsilon_n - \lambda_{\min}(\Sigma)\} \vee 0]I_p$ . For all positive integer  $r$  and all positive real number  $\epsilon_n > 0$ ,*

$$\|\Sigma^{(\epsilon_n)} - \Sigma_0\|^r \leq 2^{2r-1}\|\Sigma - \Sigma_0\|^r + 4^{r-1}|\epsilon_n|^r.$$

*Proof.* By Lemma 4.14 in Lee et al. (2020), we have

$$\begin{aligned} \lambda_{\min}(\Sigma) &= \lambda_{\min}(\Sigma - \Sigma_0 + \Sigma_0) \\ &\geq \lambda_{\min}(\Sigma_0) - \|\Sigma - \Sigma_0\|. \end{aligned}$$

Using this inequality, we get

$$\begin{aligned} \|\Sigma - \Sigma_0\| &\geq \|\Sigma - \Sigma_0\|I(\lambda_{\min}(\Sigma) < 0) \\ &\geq \{\|\Sigma - \Sigma_0\| - \lambda_{\min}(\Sigma_0)\}I(\lambda_{\min}(\Sigma) < 0) \\ &\geq -\lambda_{\min}(\Sigma)I(\lambda_{\min}(\Sigma) < 0). \end{aligned} \tag{3}$$

We also have

$$\begin{aligned} \{\epsilon_n - \lambda_{\min}(\Sigma)\} \vee 0 &\leq \{\epsilon_n - \lambda_{\min}(\Sigma)I(\lambda_{\min}(\Sigma) < 0)\} \vee 0 \\ &= \epsilon_n - \lambda_{\min}(\Sigma)I(\lambda_{\min}(\Sigma) < 0). \end{aligned} \tag{4}$$

Thus, we have

$$\begin{aligned}
\|\Sigma^{(\epsilon_n)} - \Sigma_0\|^r &= \|\Sigma - \Sigma_0 + [\{\epsilon_n - \lambda_{\min}(\Sigma)\} \vee 0]I_p\|^r \\
&\leq 2^{r-1}\|\Sigma - \Sigma_0\|^r + 2^{r-1}|\epsilon_n - \lambda_{\min}(\Sigma)I(\lambda_{\min}(\Sigma) < 0)|^r \\
&\leq 2^{r-1}\|\Sigma - \Sigma_0\|^r + 4^{r-1}|\epsilon_n|^r + 4^{r-1}|\lambda_{\min}(\Sigma)I(\lambda_{\min}(\Sigma) < 0)|^r \\
&\leq 2^{r-1}\|\Sigma - \Sigma_0\|^r + 4^{r-1}|\epsilon_n|^r + 4^{r-1}\|\Sigma - \Sigma_0\|^r \\
&\leq 2^{2r-1}\|\Sigma - \Sigma_0\|^r + 4^{r-1}|\epsilon_n|^r,
\end{aligned}$$

where the first and third inequalities are satisfied inequalities (4) and (3), respectively.  $\square$

*Proof of Theorem 2.2.* We have

$$\begin{aligned}
&E(\|\Sigma_{0,YX}\Sigma_{0,XX}^{-1} - \psi\{T_k^{(\epsilon_n)}(S_n)\}\|^2) \\
&\leq 2E(\|T_k^{(\epsilon_n)}(S_n)_{YX} - \Sigma_{0,YX}\|^2\|T_k^{(\epsilon_n)}(S_n)_{XX}^{-1}\|^2) \\
&\quad + 2\|\Sigma_{0,YX}\|^2E(\|T_k^{(\epsilon_n)}(S_n)_{XX}^{-1} - \Sigma_{0,XX}^{-1}\|^2) \\
&\leq \frac{2^3}{M_1^2}E(\|T_k^{(\epsilon_n)}(S_n)_{YX} - \Sigma_{0,YX}\|^2I[\lambda_{\min}\{T_k(S_n)_{XX}\} > M_1/2]) \tag{5}
\end{aligned}$$

$$+ \frac{2}{\epsilon_n^2}E(\|T_k^{(\epsilon_n)}(S_n)_{YX} - \Sigma_{0,YX}\|^2I[\lambda_{\min}\{T_k(S_n)_{XX}\} \leq M_1/2]) \tag{6}$$

$$+ 2M_0^2E(\|T_k^{(\epsilon_n)}(S_n)_{XX}^{-1} - \Sigma_{0,XX}^{-1}\|^2), \tag{7}$$

where the last inequality holds since  $\lambda_{\min}\{T_k^{(\epsilon_n)}(S_n)_{XX}\} \geq \lambda_{\min}\{T_k^{(\epsilon_n)}(S_n)\} \geq \epsilon_n$ . We have that there exists some positive constant  $C_1$  depending only on  $M$ ,  $M_0$ ,  $M_1$  and  $\alpha$  such that

$$\begin{aligned}
(5) &\leq \frac{2^3}{M_1^2}E(\|T_k^{(\epsilon_n)}(S_n) - \Sigma_0\|^2) \\
&\leq \frac{2^3}{M_1^2}\{2^3E(\|T_k(S_n) - \Sigma_0\|^2) + 4\epsilon_n^2\} \\
&\leq C_1\left\{\frac{k + \log p}{n} + k^{-2\alpha} + \epsilon_n^2\right\},
\end{aligned}$$

for all sufficiently large  $n$ . The second and last inequalities hold by Lemma 2.1 and Theorem 2 of Cai and Zhou (2010), respectively. By Lemmas A.2 and A.3, there exist some

positive constants  $C_2$  and  $\lambda_1$  depending only on  $M_0$  and  $M_1$  such that

$$\begin{aligned} (6) &\leq \frac{2}{\epsilon_n^2} E(\|T_k^{(\epsilon_n)}(S_n) - \Sigma_0\|^4)^{1/2} P(\lambda_{\min}(T_k(S_n)_{XX}) \leq M_1/2)^{1/2} \\ &\leq \frac{C_2}{\epsilon_n^2} p^{1/2} 5^{k/2} \exp(-\lambda_1 n), \end{aligned}$$

for all sufficiently large  $n$ . Finally, by Lemma A.4, we get the upper bound of (7) as

$$(7) \leq C_3 \left( \frac{k + \log p}{n} + k^{-2\alpha} + \epsilon_n^2 + \frac{p^{1/2} 5^{k/2} \exp(-\lambda_2 n)}{\epsilon_n^2} \right),$$

for some positive constants  $C_3$  and  $\lambda_2$  depending only on  $M$ ,  $M_0$ ,  $M_1$  and  $\alpha$ . Combining the upper bounds of (5), (6) and (7), we complete the proof.  $\square$

### 3 Proof of Lemma 3

In this section, we prove the Lemma 2.3. For this proof, we present Lemma 3.1.

**Lemma 3.1.** *Let  $q$  and  $k$  be positive integers with  $k < q$ , and  $A \in \mathcal{C}_q$  be a  $k$ -band matrix. For positive real numbers  $a$  and  $b$  with  $q > \lfloor ak \log k \rfloor + \lfloor bk \log k \rfloor$ , we express  $A$  and  $A^{-1}$  as*

$$A = \begin{bmatrix} A_{11} & A_{12} \\ A_{21} & A_{22} \end{bmatrix}, A^{-1} = \Omega = \begin{bmatrix} \Omega_{11} & \Omega_{12} \\ \Omega_{21} & \Omega_{22} \end{bmatrix},$$

where  $A_{22}, \Omega_{22} \in \mathbb{R}^{(\lfloor ak \log k \rfloor + \lfloor bk \log k \rfloor) \times (\lfloor ak \log k \rfloor + \lfloor bk \log k \rfloor)}$ . There exist some positive constants  $\lambda$  and  $C$  depending only on  $\|A\|$  and  $\|A^{-1}\|$  such that

$$\|M_{\lfloor ak \log k \rfloor + 1}^{(\lfloor bk \log k \rfloor)}(\Omega_{22}) - M_{\lfloor ak \log k \rfloor + 1}^{(\lfloor bk \log k \rfloor)}(A_{22}^{-1})\| \leq C k^{-a\lambda + 1},$$

for all sufficiently large  $k$  and  $q$  with  $\lfloor ak \log k \rfloor \geq k$  and  $q > \lfloor ak \log k \rfloor + \lfloor bk \log k \rfloor$ .

*Proof.* Let  $\{B_{\lfloor ak \log k \rfloor}(\Omega)\}_{12} = \{B_{\lfloor ak \log k \rfloor}(\Omega)\}_{1:q^*, (q^*+1):q}$ , where  $q^* = q - \lfloor ak \log k \rfloor - \lfloor bk \log k \rfloor$  and  $B_{\lfloor ak \log k \rfloor}$  is  $\lfloor ak \log k \rfloor$ -banding operator defined in Bickel and Levina (2008).

First, we show the equality

$$M_{\lfloor ak \log k \rfloor + 1}^{(\lfloor bk \log k \rfloor)}(A_{22}^{-1}[I - A_{21}\{B_{\lfloor ak \log k \rfloor}(\Omega)\}_{12}]) = M_{\lfloor ak \log k \rfloor + 1}^{(\lfloor bk \log k \rfloor)}(A_{22}^{-1}). \quad (8)$$

Since  $\lfloor ak \log k \rfloor \geq k$  and  $A$  is a  $k$ -band matrix,  $A_{21}$  is expressed as

$$A_{21} = \begin{bmatrix} O_{\{\lfloor ak \log k \rfloor \times (q^* - \lfloor ak \log k \rfloor)\}} & A^* \\ O_{\{\lfloor bk \log k \rfloor \times (q^* - \lfloor ak \log k \rfloor)\}} & O_{(\lfloor bk \log k \rfloor \times \lfloor ak \log k \rfloor)} \end{bmatrix},$$

for some  $\lfloor ak \log k \rfloor \times \lfloor ak \log k \rfloor$ -matrix  $A^*$ . Likewise,  $\{B_{\lfloor ak \log k \rfloor}(\Omega)\}_{12}$  is expressed as

$$\{B_{\lfloor ak \log k \rfloor}(\Omega)\}_{12} = \begin{bmatrix} O_{\{(q^* - \lfloor ak \log k \rfloor) \times \lfloor ak \log k \rfloor\}} & O_{\{(q^* - \lfloor ak \log k \rfloor) \times \lfloor bk \log k \rfloor\}} \\ B_{(\lfloor ak \log k \rfloor \times \lfloor ak \log k \rfloor)}^* & O_{(\lfloor ak \log k \rfloor \times \lfloor bk \log k \rfloor)} \end{bmatrix},$$

for some  $\lfloor ak \log k \rfloor \times \lfloor ak \log k \rfloor$ -matrix  $B^*$ . Thus,

$$A_{21}\{B_{\lfloor ak \log k \rfloor}(\Omega)\}_{12} = \begin{bmatrix} A^* B^* & O_{(\lfloor ak \log k \rfloor \times \lfloor bk \log k \rfloor)} \\ O_{(\lfloor bk \log k \rfloor \times \lfloor ak \log k \rfloor)} & O_{(\lfloor bk \log k \rfloor \times \lfloor bk \log k \rfloor)} \end{bmatrix},$$

and  $M_{\lfloor ak \log k \rfloor + 1}^{(\lfloor bk \log k \rfloor)}(A_{22}^{-1}[A_{21}\{B_{\lfloor ak \log k \rfloor}(\Omega)\}_{12}])$  is the zero matrix, which gives the equality (8).

Next, we show the upper bound of

$$\|M_{\lfloor ak \log k \rfloor + 1}^{(\lfloor bk \log k \rfloor)}(A_{22}^{-1}[I - A_{21}\{B_{\lfloor ak \log k \rfloor}(\Omega)\}_{12}]) - M_{\lfloor ak \log k \rfloor + 1}^{(\lfloor bk \log k \rfloor)}(\Omega_{22})\|. \quad (9)$$

By the block matrix inversion formula,  $\Omega_{22} = A_{22}^{-1}(I - A_{21}\Omega_{12})$ , we have

$$\begin{aligned} (9) &= \|M_{\lfloor ak \log k \rfloor + 1}^{(\lfloor bk \log k \rfloor)}(A_{22}^{-1}A_{21}[\{B_{\lfloor ak \log k \rfloor}(\Omega)\}_{12} - \Omega_{12}])\| \\ &\leq \|A_{22}^{-1}A_{21}\| \|\{B_{\lfloor ak \log k \rfloor}(\Omega)\}_{12} - \Omega_{12}\| \\ &\leq \lambda_{\min}(A_{22})^{-1} \|A_{21}\| \|B_{\lfloor ak \log k \rfloor}(\Omega) - \Omega\|_1 \\ &\leq \|A\| \|A^{-1}\| \|B_{\lfloor ak \log k \rfloor}(\Omega) - \Omega\|_1. \end{aligned}$$

By Lemma 1.1, there exist some positive constants  $\lambda_1$  and  $C_1$  depending only on  $\|A\|$  and  $\|A^{-1}\|$  such that

$$\|B_{\lfloor ak \log k \rfloor}(\Omega) - \Omega\|_1 \leq C_1 k^{-a\lambda_1 + 1},$$

for all sufficiently large  $k$  with  $p > k \vee (ak \log k)$ . By combining this inequality with the equality (8), we get

$$\|M_{\lfloor ak \log k \rfloor + 1}^{(\lfloor bk \log k \rfloor)}(A_{22}^{-1}) - M_{\lfloor ak \log k \rfloor + 1}^{(\lfloor bk \log k \rfloor)}(\Omega_{22})\| \leq C_1 \|A\| \|A^{-1}\| k^{-a\lambda_1 + 1},$$

for all sufficiently large  $k$ . □

Next, we prove Lemma 2.3.

*Proof of Lemma 2.3.* There exist some positive constants  $C_1$  and  $C_2$  depending only on  $M$ ,  $M_0$  and  $M_1$  such that

$$\begin{aligned}
& \|\psi(\Sigma_0) - T_k(\Sigma_0)_{YX} T_k(\Sigma_{0,XX})^{-1}\| \\
& \leq \|\Sigma_{0,XX}^{-1}\| \|T_k(\Sigma_0)_{YX} - \Sigma_{0,YX}\| \\
& \quad + \|T_k(\Sigma_0)_{YX}\| \|\Sigma_{0,XX}^{-1} - T_k(\Sigma_{0,XX})^{-1}\| \\
& \leq M_1^{-1} M (\lfloor k/2 \rfloor)^{-\alpha} + (\|\Sigma_0\| + \|T_k(\Sigma_0) - \Sigma_0\|) \|\Sigma_{0,XX}^{-1} - T_k(\Sigma_{0,XX})^{-1}\| \\
& \leq M_1^{-1} M (\lfloor k/2 \rfloor)^{-\alpha} + \{M_0 + M (\lfloor k/2 \rfloor)^{-\alpha}\} C_1 (\lfloor k/2 \rfloor)^{-\alpha} \\
& \leq C_2 (\lfloor k/2 \rfloor)^{-\alpha},
\end{aligned}$$

for all sufficiently large  $k$ . The third inequality holds by Lemma A.1 since  $\Sigma_{0,XX} \in \mathcal{F}_{p_0, \alpha}(M, M_0, M_1)$ . Then, we have

$$\begin{aligned}
& \|\psi(\Sigma_0) - T_k(\Sigma_0)_{YX} \Lambda^{(0)}\{T_k(\Sigma_{0,XX}); 2\lfloor ak \log k \rfloor\}\| \\
& \leq \|\psi(\Sigma_0) - T_k(\Sigma_0)_{YX} T_k(\Sigma_{0,XX})^{-1}\| \\
& \quad + \|T_k(\Sigma_0)_{YX} [\Lambda^{(0)}\{T_k(\Sigma_{0,XX}); 2\lfloor ak \log k \rfloor\} - T_k(\Sigma_{0,XX})^{-1}]\| \\
& \leq C_2 (\lfloor k/2 \rfloor)^{-\alpha} + \|T_k(\Sigma_0)_{YX} [\Lambda^{(0)}\{T_k(\Sigma_{0,XX}); 2\lfloor ak \log k \rfloor\} - T_k(\Sigma_{0,XX})^{-1}]\|.
\end{aligned}$$

For this upper bound, we have

$$\begin{aligned}
& \|T_k(\Sigma_0)_{YX} [\Lambda^{(0)}\{T_k(\Sigma_{0,XX}); 2\lfloor ak \log k \rfloor\} - T_k(\Sigma_{0,XX})^{-1}]\| \\
& \leq \|T_k(\Sigma_0)_{YX} [T_k(\Sigma_{0,XX})^{-1} - M_{p_0 - \lfloor ak \log k \rfloor + 1}^{*(\lfloor ak \log k \rfloor)} \{T_k(\Sigma_{0,XX})^{-1}\}]\| \tag{10}
\end{aligned}$$

$$+ \|T_k(\Sigma_0)_{YX} [M_{p_0 - \lfloor ak \log k \rfloor + 1}^{*(\lfloor ak \log k \rfloor)} \{T_k(\Sigma_{0,XX})^{-1}\} - \Lambda^{(0)}\{T_k(\Sigma_{0,XX}); 2\lfloor ak \log k \rfloor\}]\| \tag{11}$$

First, we show the upper bound of (10). Since  $T_k(\Sigma_0)$  is a  $k$ -band matrix,  $T_k(\Sigma_0)_{YX}$  is expressed as

$$T_k(\Sigma_0)_{YX} = \begin{bmatrix} O_{k \times (p_0 - k)} & \{T_k(\Sigma_0)_{YX}\}_{1:k, (p_0 - k + 1):p_0} \\ O_{(p - p_0 - k) \times (p_0 - k)} & O_{(p - p_0 - k) \times k} \end{bmatrix}. \tag{12}$$

Since  $\lfloor ak \log k \rfloor \geq k$ , the definition of  $M_{p_0 - \lfloor ak \log k \rfloor + 1}^{*(\lfloor ak \log k \rfloor)}$  gives

$$= \begin{bmatrix} T_k(\Sigma_{0,XX})^{-1} - M_{p_0 - \lfloor ak \log k \rfloor + 1}^{*(\lfloor ak \log k \rfloor)} \{T_k(\Sigma_{0,XX})^{-1}\} & C^* \\ \{T_k(\Sigma_{0,XX})^{-1}\}_{(p_0-k+1):p_0, 1:(p_0 - \lfloor ak \log k \rfloor)} & O_{k \times \lfloor ak \log k \rfloor} \end{bmatrix},$$

for some  $(p_0 - k) \times (p_0 - \lfloor ak \log k \rfloor)$ -matrix  $B^*$  and some  $(p_0 - k) \times \lfloor ak \log k \rfloor$ -matrix  $C^*$ .

Thus,

$$= \begin{bmatrix} T_k(\Sigma_0)_{YX} [T_k(\Sigma_{0,XX})^{-1} - M_{p_0 - \lfloor ak \log k \rfloor + 1}^{*(\lfloor ak \log k \rfloor)} \{T_k(\Sigma_{0,XX})^{-1}\}] & O_{k \times \lfloor ak \log k \rfloor} \\ \{T_k(\Sigma_0)_{YX}\}_{1:k, (p_0-k+1):p_0} \{T_k(\Sigma_{0,XX})^{-1}\}_{(p_0-k+1):p_0, 1:(p_0 - \lfloor ak \log k \rfloor)} & O_{(p-p_0-k) \times \lfloor ak \log k \rfloor} \\ O_{(p-p_0-k) \times (p_0 - \lfloor ak \log k \rfloor)} & O_{(p-p_0-k) \times \lfloor ak \log k \rfloor} \end{bmatrix},$$

and

$$\begin{aligned} (10) &= \|\{T_k(\Sigma_0)_{YX}\}_{1:k, (p_0-k+1):p_0} \{T_k(\Sigma_{0,XX})^{-1}\}_{(p_0-k+1):p_0, 1:(p_0 - \lfloor ak \log k \rfloor)}\| \\ &\leq \|T_k(\Sigma_0)_{YX}\| \|\{T_k(\Sigma_{0,XX})^{-1}\}_{(p_0-k+1):p_0, 1:(p_0 - \lfloor ak \log k \rfloor)}\|. \end{aligned}$$

Let  $\{T_k(\Sigma_{0,XX})\}^{-1} = (b_{ij})_{1 \leq i, j \leq p_0}$ . Every element  $b_{ij}$  in  $\{T_k(\Sigma_{0,11})^{-1}\}_{(p_0-k+1):p_0, 1:(p_0 - \lfloor ak \log k \rfloor)}$  satisfies

$$\begin{aligned} |i - j| &\geq \lfloor ak \log k \rfloor - k + 1 \\ &> \lfloor ak \log k \rfloor / 2, \end{aligned}$$

since  $\lfloor ak \log k \rfloor / 2 \geq k$ . Thus, by Lemma 1.1, there exist some positive constants  $C_3$  and  $\lambda_1$  depending only on  $M_0$  and  $M_1$  such that

$$\begin{aligned} &\|\{T_k(\Sigma_{0,XX})^{-1}\}_{(p_0-k+1):p_0, 1:(p_0 - \lfloor ak \log k \rfloor)}\|_2 \\ &\leq \|\{T_k(\Sigma_{0,XX})^{-1}\}_{(p_0-k+1):p_0, 1:(p_0 - \lfloor ak \log k \rfloor)}\|_1 \vee \|\{T_k(\Sigma_{0,XX})^{-1}\}_{(p_0-k+1):p_0, 1:(p_0 - \lfloor ak \log k \rfloor)}\|_\infty \\ &\leq C_3 k^{-a\lambda_1 + 1}, \end{aligned}$$

for all sufficiently large  $k$  with  $p_0 > k \vee \lfloor ak \log k \rfloor / 2$ . Since

$$\|T_k(\Sigma_0)_{YX}\| \leq \|\Sigma_0\| + \|\Sigma_0 - T_k(\Sigma_0)\| \leq M_0 + M \lfloor k/2 \rfloor,$$



we get

$$(10) \leq (M_0 + M\lfloor k/2 \rfloor)C_2k^{-a\lambda_1+1}, \quad (13)$$

for all sufficiently large  $k$  with  $p_0 > k \vee \lfloor ak \log k \rfloor / 2$ .

Next, we show the upper bound of (11). Since  $T_k(\Sigma_0)_{YX}$  is expressed as (12), we have

$$(11) \leq \|T_k(\Sigma_0)\| \| [M_{p_0-\lfloor ak \log k \rfloor+1}^{*(\lfloor ak \log k \rfloor)} \{T_k(\Sigma_{0,XX})^{-1}\} - \Lambda^{(0)}\{T_k(\Sigma_{0,XX}); 2\lfloor ak \log k \rfloor\}]_{(p_0-k+1):p_0, 1:p_0} \| \quad (14)$$

Note

$$\begin{aligned} & [M_{p_0-\lfloor ak \log k \rfloor+1}^{*(\lfloor ak \log k \rfloor)} \{T_k(\Sigma_{0,XX})^{-1}\} - \Lambda^{(0)}\{T_k(\Sigma_{0,XX}); 2\lfloor ak \log k \rfloor\}]_{(p_0-k+1):p_0, 1:p_0} \\ &= \begin{bmatrix} O_{k \times (p_0-2\lfloor ak \log k \rfloor)} & -D_1^* & D_3^* - D_2^* \end{bmatrix}, \end{aligned}$$

where  $D_1^*$ ,  $D_2^*$  and  $D_3^*$  are  $k \times \lfloor ak \log k \rfloor$ -matrices with

$$\begin{aligned} D_1^* &= [M_{p_0-2\lfloor ak \log k \rfloor+1}^{(2\lfloor ak \log k \rfloor)} \{T_k(\Sigma_{0,XX})\}^{-1}]_{(2\lfloor ak \log k \rfloor-k+1):2\lfloor ak \log k \rfloor, 1:\lfloor ak \log k \rfloor} \\ D_2^* &= [M_{p_0-2\lfloor ak \log k \rfloor+1}^{(2\lfloor ak \log k \rfloor)} \{T_k(\Sigma_{0,XX})\}^{-1}]_{(2\lfloor ak \log k \rfloor-k+1):2\lfloor ak \log k \rfloor, (\lfloor ak \log k \rfloor+1):2\lfloor ak \log k \rfloor} \\ D_3^* &= \{T_k(\Sigma_{0,XX})^{-1}\}_{(p_0-k+1):p_0, (p_0-\lfloor ak \log k \rfloor+1):p_0}. \end{aligned}$$

We have

$$(11) \leq \|T_k(\Sigma_0)\| (\|D_1^*\| + \|D_2^* - D_3^*\|).$$

First, we show the upper bound of  $\|D_2^* - D_3^*\|$ . Let

$$\begin{aligned} A_{22} &= M_{p_0-2\lfloor ak \log k \rfloor+1}^{(2\lfloor ak \log k \rfloor)} \{T_k(\Sigma_{0,XX})\} \\ \Omega_{22} &= M_{p_0-2\lfloor ak \log k \rfloor+1}^{(2\lfloor ak \log k \rfloor)} \{T_k(\Sigma_{0,XX})^{-1}\}. \end{aligned}$$

By Lemma 3.1, there exist some positive constants  $C_4$  and  $\lambda_2$  depending only on  $M_0$  and  $M_1$  such that

$$\begin{aligned} \|D_2^* - D_3^*\| &\leq \|M_{\lfloor ak \log k \rfloor+1}^{(\lfloor ak \log k \rfloor)}(\Omega_{22}) - M_{\lfloor ak \log k \rfloor+1}^{(\lfloor ak \log k \rfloor)}(A_{22}^{-1})\| \\ &\leq C_3k^{-a\lambda_2+1}, \end{aligned}$$

for all sufficiently large  $k$  with  $\lfloor ak \log k \rfloor \geq k$  and  $p_0 > 2\lfloor ak \log k \rfloor$ .

Next, we show the upper bound of  $\|D_1^*\|$ . Let  $M_{p_0-2\lfloor ak \log k \rfloor+1}^{(2\lfloor ak \log k \rfloor)} \{T_k(\Sigma_{0,XX})\}^{-1} = (c_{ij})_{1 \leq i,j \leq 2\lfloor ak \log k \rfloor}$ . Every element  $c_{ij}$  in  $D_1^*$  satisfies

$$\begin{aligned} |i - j| &\geq \lfloor ak \log k \rfloor - k + 1 \\ &\geq \lfloor ak \log k \rfloor / 2, \end{aligned}$$

since  $\lfloor ak \log k \rfloor / 2 \geq k$ . Thus, Lemma 1.1 gives that there exist some positive constants  $C_5$  and  $\lambda_3$  depending only on  $M_0$  and  $M_1$  such that

$$\|D_1^*\| \leq C_5 k^{-a\lambda_3+1},$$

for all sufficiently large  $k$  with  $p_0 > k \vee (ak \log k)$ . By combining this inequality with (14), we have

$$(11) \leq (M_0 + M(\lfloor k/2 \rfloor)^{-\alpha})(C_2 k^{-a\lambda_2+1} + C_3 k^{-a\lambda_3+1}). \quad (15)$$

By collecting the inequalities (13) and (15), the proof is completed.  $\square$

## 4 Proofs of Theorems 6 and 7

In this section, we prove Theorems 3.1 and 3.2 which give the P-risk convergence rates of the tapering and blockwise tapering post-processed posteriors, respectively. First, we present Lemmas 4.1-4.4 necessary for the proofs of Theorems 3.1 and 3.2.

**Lemma 4.1.** *Let  $k$  and  $p$  be positive integers with  $k \leq p$ . Suppose  $\Sigma_0 \in \mathcal{F}_{p,\alpha}(M, M_0, M_1)$ , and let the prior  $\pi^i$  of  $\Sigma$  be  $IW_p(A_n, \nu_n)$  for  $A_n \in \mathcal{C}_p$  and  $\nu_n > 2p$ . If  $k \vee \|A_n\| \vee (\nu_n - 2p) \vee \log p = o(n)$  and  $\epsilon_n = O(1)$ , then for all sufficiently large  $n$ ,  $E_{\Sigma_0} \{E^{\pi^i}(\|T_k^{(\epsilon_n)}(\Sigma) - \Sigma_0\|^4 \mid \mathbb{Z}_n)\}$  is bounded above by some positive constant depending only on  $M, M_0, M_1$  and  $\alpha$ .*

The proof of this lemma is given in Section 6.

**Lemma 4.2.** *Suppose the same setting of Lemma 4.1. If  $c \leq \lambda_{\min}(\Sigma_0)/2$ ,  $\lfloor k/2 \rfloor > \{4M/\lambda_{\min}(\Sigma_0)\}^{1/\alpha}$  and  $k \vee \|A_n\| \vee (\nu_n - 2p) \vee \log p = o(n)$ , then there exist some positive constants  $C$  and  $\lambda$  depending only on  $M_0$  and  $M_1$  such that*

$$E_{\Sigma_0}(P^{\pi^i}[\lambda_{\min}\{T_k(\Sigma)\} \leq c \mid \mathbb{Z}_n]) \leq Cp5^k \exp(-\lambda n),$$

for all sufficiently large  $n$ .

The proof of this lemma is given in Section 6.

**Lemma 4.3.** *Suppose the same setting of Lemma 4.1. If  $\|A_n\| \vee (\nu_n - 2p) \vee k \vee \log p = o(n)$  and  $\epsilon_n = O(1)$ , then there exist some positive constant  $C$  depending only on  $M$ ,  $M_0$ ,  $M_1$  and  $\alpha$  such that*

$$E_{\Sigma_0}\{E^{\pi^i}(\|\Sigma_0 - T_k^{(\epsilon_n)}(\Sigma)\|^2 \mid \mathbb{Z}_n)\} \leq C\left(k^{-2\alpha} + \frac{k + \log p}{n} + \epsilon_n^2\right),$$

for sufficiently large  $n$ .

The proof of this lemma is given in Section 6.

**Lemma 4.4.** *Suppose the same setting of Lemma 4.1. Let  $q$  and  $k$  be positive constants with  $k < q \leq p$ , and let  $\{T_k^{(\epsilon_n)}(\Sigma)\}_{1:q,1:q}$  and  $(\Sigma_0)_{1:q,1:q}$  be denoted by  $T_k^{(\epsilon_n)}(\Sigma)_{11}$  and  $\Sigma_{0,11}$ , respectively. If  $\lfloor k/2 \rfloor > \{4M/\lambda_{\min}(\Sigma_0)\}^{1/\alpha}$  and  $k \vee \|A_n\| \vee (\nu_n - 2p) \vee \log p = o(n)$ , then there exist positive constants  $C$  and  $\lambda$  depending only on  $M$ ,  $M_0$ ,  $M_1$  and  $\alpha$  such that*

$$E_{\Sigma_0}\{E^{\pi^i}(\|\Sigma_{0,11}^{-1} - T_k^{(\epsilon_n)}(\Sigma)_{11}^{-1}\|^2 \mid \mathbb{Z}_n)\} \leq C\left\{\frac{k + \log p}{n} + k^{-2\alpha} + \epsilon_n^2 + \frac{p^{1/2}5^{k/2} \exp(-\lambda n)}{\epsilon_n^2}\right\},$$

for all sufficiently large  $n$ .

The proof of this lemma is given in Section 6.

Now we prove Theorems 3.1 and 3.2.

*Proof of Theorem 3.1.* Since  $\lambda_{\min}\{T_k^{(\epsilon_n)}(\Sigma)_{XX}^{-1}\} \geq \lambda_{\min}\{T_k^{(\epsilon_n)}(\Sigma)^{-1}\} \geq \epsilon_n$ , we have

$$\begin{aligned}
& E_{\Sigma_0}\{E^{\pi^i}(\|\psi(\Sigma_0) - \psi\{T_k^{(\epsilon_n)}(\Sigma)\}\|^2 \mid \mathbb{Z}_n)\} \\
&= E_{\Sigma_0}\{E^{\pi^i}(\|\Sigma_{0,YX}\Sigma_{0,XX}^{-1} - T_k^{(\epsilon_n)}(\Sigma)_{YX}T_k^{(\epsilon_n)}(\Sigma)_{XX}^{-1}\|^2 \mid \mathbb{Z}_n)\} \\
&\leq 2E_{\Sigma_0}\{E^{\pi^i}(\|T_k^{(\epsilon_n)}(\Sigma)_{YX} - \Sigma_{0,YX}\|^2\|T_k^{(\epsilon_n)}(\Sigma)_{XX}^{-1}\|^2 \mid \mathbb{Z}_n)\} \\
&\quad + 2\|\Sigma_{0,YX}\|^2 E_{\Sigma_0}\{E^{\pi^i}(\|T_k^{(\epsilon_n)}(\Sigma)_{XX}^{-1} - \Sigma_{0,XX}^{-1}\|^2 \mid \mathbb{Z}_n)\} \\
&\leq \frac{2^3}{M_1^2} E_{\Sigma_0}\{E^{\pi^i}(\|T_k^{(\epsilon_n)}(\Sigma)_{YX} - \Sigma_{0,YX}\|^2 \mid \mathbb{Z}_n)\} \tag{16}
\end{aligned}$$

$$\begin{aligned}
& + \frac{2}{\epsilon_n^2} E_{\Sigma_0}\{E^{\pi^i}(\|T_k^{(\epsilon_n)}(\Sigma)_{YX} - \Sigma_{0,YX}\|^2 I[\lambda_{\min}\{T_k(S_n)\} \leq M_1/2] \mid \mathbb{Z}_n)\} \tag{17}
\end{aligned}$$

$$\begin{aligned}
& + 2\|\Sigma_{0,YX}\|^2 E_{\Sigma_0}\{E^{\pi^i}(\|T_k^{(\epsilon_n)}(\Sigma)_{XX}^{-1} - \Sigma_{0,XX}^{-1}\|^2 \mid \mathbb{Z}_n)\}. \tag{18}
\end{aligned}$$

Lemmas 4.3 and 4.4 give that there exist some positive constants  $C_1$  and  $\lambda_1$  depending only on  $M$ ,  $M_0$ ,  $M_1$  and  $\alpha$  such that

$$(16) + (18) \leq C_1 \left\{ \frac{k + \log p}{n} + k^{-2\alpha} + \epsilon_n^2 + \frac{p^{1/2}5^{k/2} \exp(-\lambda_1 n)}{\epsilon_n^2} \right\},$$

for all sufficiently large  $n$ . Next we show the upper bound of (17). By Lemmas 4.1 and 4.2, there exist positive constants  $C_2$  and  $\lambda_2$  depending only on  $M$ ,  $M_0$ ,  $M_1$  and  $\alpha$  such that

$$\begin{aligned}
(17) &\leq \frac{2}{\epsilon_n^2} E_{\Sigma_0}\{E^{\pi^i}(\|T_k^{(\epsilon_n)}(\Sigma)_{YX} - \Sigma_{0,YX}\|^4 \mid \mathbb{Z}_n)\}^{1/2} \\
&\quad \times E_{\Sigma_0}\{P^{\pi^i}(I[\lambda_{\min}\{T_k(S_n)\} \leq M_1/2] \mid \mathbb{Z}_n)\}^{1/2} \\
&\leq C_2 \frac{p^{1/2}5^{k/2}}{\epsilon_n^2} \exp(-\lambda_2 n),
\end{aligned}$$

for all sufficiently large  $n$ . Collecting the upper bounds of (16), (17) and (18), we complete the proof. □

*Proof of Theorem 3.2.* We have

$$\begin{aligned}
& E_{\Sigma_0} \{ E^{\pi^i} (||\psi(\Sigma_0) - T_k(\Sigma)_{YX} \Lambda^{(\epsilon_n)} \{ T_k(\Sigma)_{XX}; 2 \lfloor ak \log k \rfloor \} ||^2 \mid \mathbb{Z}_n) \} \\
\leq & 2 ||\psi(\Sigma_0) - T_k(\Sigma_0)_{YX} \Lambda^{(0)} \{ T_k(\Sigma_{0,XX}); 2 \lfloor ak \log k \rfloor \} ||^2 \quad (19) \\
& + 4 E_{\Sigma_0} \{ E^{\pi^i} (||\{ T_k(\Sigma_0)_{YX} - T_k(\Sigma)_{YX} \} \Lambda^{(\epsilon_n)} \{ T_k(\Sigma)_{XX}; 2 \lfloor ak \log k \rfloor \} ||^2 \mid \mathbb{Z}_n) \} \quad (20) \\
& + 4 ||T_k(\Sigma_0)_{YX} ||^2 E_{\Sigma_0} \{ E^{\pi^i} ( \Lambda^{(0)} \{ T_k(\Sigma_{0,XX}); 2 \lfloor ak \log k \rfloor \} \\
& - \Lambda^{(\epsilon_n)} \{ T_k(\Sigma)_{XX}; 2 \lfloor ak \log k \rfloor \} ||^2 \mid \mathbb{Z}_n) \}. \quad (21)
\end{aligned}$$

Lemma 2.3 gives that there exist positive constants  $C_1$  and  $\lambda_1$  depending only on  $M$ ,  $M_0$ ,  $M_1$  and  $\alpha$  such that

$$(19) \leq C_1 k^{-2\{\alpha \wedge (a\lambda_1 - 1)\}}$$

for all sufficiently large  $k$  with  $\lfloor ak \log k \rfloor / 2 > k$  and  $p_0 > 2 \lfloor ak \log k \rfloor$ . Let  $\tilde{M} = M_{p_0 - 2 \lfloor ak \log k \rfloor + 1}^{(2 \lfloor ak \log k \rfloor)}$  in this proof. By the definition of  $\Lambda^{(\epsilon_n)}$ , we have

$$||\Lambda^{(\epsilon_n)} \{ T_k(\Sigma_{XX}); 2 \lfloor ak \log k \rfloor \} || = ||T_k^{(\epsilon_n)} \{ \tilde{M}(\Sigma_{XX}) \}^{-1} ||.$$

Thus, there exist positive constants  $C_2$  and  $\lambda_2$  depending only on  $M$ ,  $M_0$ ,  $M_1$  and  $\alpha$  such that

$$\begin{aligned}
(20) & \leq 4 E_{\Sigma_0} \{ E^{\pi^i} (||T_k(\Sigma_0)_{YX} - T_k(\Sigma)_{YX} ||^2 ||T_k^{(\epsilon_n)} \{ \tilde{M}(\Sigma_{XX}) \}^{-1} ||^2 \mid \mathbb{Z}_n) \} \\
& \leq \frac{4}{\epsilon_n^2} E_{\Sigma_0} \{ E^{\pi^i} (||T_k(\Sigma_0)_{YX} - T_k(\Sigma)_{YX} ||^2 I[\lambda_{\min} \{ \tilde{M}(\Sigma_{XX}) \} < M_1/2] \mid \mathbb{Z}_n) \} \\
& \quad + \frac{16}{M_1^2} E_{\Sigma_0} \{ E^{\pi^i} (||T_k(\Sigma_0)_{YX} - T_k(\Sigma)_{YX} ||^2 \mid \mathbb{Z}_n) \} \\
& \leq \frac{4}{\epsilon_n^2} E_{\Sigma_0} \{ E^{\pi^i} (||T_k(\Sigma_0) - T_k(\Sigma) ||^4 \mid \mathbb{Z}_n) \}^{1/2} E_{\Sigma_0} [P^{\pi^i} \{ \lambda_{\min}(\Sigma) < M_1/2 \mid \mathbb{Z}_n \}]^{1/2} \\
& \quad + \frac{16}{M_1^2} E_{\Sigma_0} \{ E^{\pi^i} (||T_k(\Sigma_0)_{YX} - T_k(\Sigma)_{YX} ||^2 \mid \mathbb{Z}_n) \} \\
& \leq C_2 \left( \frac{1}{\epsilon_n^2} p^{1/2} 5^{k/2} \exp(-\lambda_2 n) + \frac{k + \log p}{n} + k^{-2\alpha} \right),
\end{aligned}$$

for all sufficiently large  $n$ . The third inequality holds since  $\lambda_{\min} \{ \tilde{M}(\Sigma_{XX}) \} \geq \lambda_{\min}(\Sigma)$ . The last inequality holds by Lemma 4.1, 4.2 and 4.3. For the upper bound of (21), we

have

$$\begin{aligned}
& E_{\Sigma_0} \{ E^{\pi^i} (\Lambda^{(0)} \{ T_k(\Sigma_{0,XX}); 2 \lfloor ak \log k \rfloor \} - \Lambda^{(\epsilon_n)} \{ T_k(\Sigma)_{XX}; 2 \lfloor ak \log k \rfloor \})^2 \mid \mathbb{Z}_n \} \\
&= E_{\Sigma_0} \{ E^{\pi^i} (\| T_k \{ \tilde{M}(\Sigma_{0,XX}) \}^{-1} - T_k^{(\epsilon_n)} \{ \tilde{M}(\Sigma_{XX}) \}^{-1} \|^2 \mid \mathbb{Z}_n) \} \\
&\leq 2 E_{\Sigma_0} \{ E^{\pi^i} (\| \tilde{M}(\Sigma_{0,XX})^{-1} - T_k^{(\epsilon_n)} \{ \tilde{M}(\Sigma_{XX}) \}^{-1} \|^2 \mid \mathbb{Z}_n) \} \tag{22} \\
&\quad + 2 \| \tilde{M}(\Sigma_{0,XX})^{-1} - T_k \{ \tilde{M}(\Sigma_{0,XX}) \}^{-1} \|^2 \tag{23}
\end{aligned}$$

where the first equality holds by the definition of  $\Lambda^{(0)}$  and  $\Lambda^{(\epsilon_n)}$ . Since  $\tilde{M}(\Sigma_{0,XX}) \in \mathcal{F}_{2 \lfloor ak \log k \rfloor, \alpha}(M, M_0, M_1)$ , Lemma A.1 gives that there exists some positive constant  $C_3$  depending only on  $M$ ,  $M_0$  and  $M_1$  such that

$$(23) \leq C_3 (\lfloor k/2 \rfloor)^{-2\alpha}$$

for all sufficiently large  $k$ . Lemma 4.4 gives that there exist some positive constants  $C_4$  and  $\lambda_3$  depending only on  $M$ ,  $M_0$ ,  $M_1$  and  $\alpha$  such that

$$(22) \leq C_4 \left\{ \frac{k + \log p}{n} + k^{-2\alpha} + \epsilon_n^2 + \frac{p^{1/2} 5^{k/2} \exp(-\lambda_3 n)}{\epsilon_n^2} \right\},$$

for all sufficiently large  $n$ . Thus, there exists some positive constant  $C_5$  depending only on  $M$ ,  $M_0$ ,  $M_1$  and  $\alpha$  such that

$$(21) \leq C_5 \left\{ \frac{k + \log p}{n} + k^{-2\alpha} + \epsilon_n^2 + \frac{p^{1/2} 5^{k/2} \exp(-\lambda_3 n)}{\epsilon_n^2} \right\},$$

for all sufficiently large  $n$  and  $k$ . Collecting the upper bounds of (19), (20) and (21), we complete the proof. □

## 5 Proofs of lemmas in Appendix A

In this section, we prove Lemmas A.1-A.5 which are presented in Appendix A. For the proofs we present Lemmas 5.1 and 5.2.

**Lemma 5.1.** *Let  $p$  and  $k$  be positive integers with  $k \leq p$ . For an arbitrary covariance matrix  $\Sigma \in \mathcal{C}_p$ ,*

$$\|T_k(\Sigma)\|_r \leq 3 \max_{1 \leq l \leq p} \|M_l^{(k)}(\Sigma)\|_r,$$

where  $\|\cdot\|_r$  is the matrix  $r$ -norm.

*Proof.* Cai and Zhou (2010) in Lemma 1 shows

$$T_k(\Sigma) = (k/2)^{-1} \{S^{*(k)}(\Sigma) - S^{*(k/2)}(\Sigma)\},$$

where  $S^{*(k)}(\Sigma) = \sum_{l=1-k}^p M_l^{*(k)}(\Sigma)$ . Thus, we have

$$\|T_k(\Sigma)\|_r \leq (2/k)(\|S^{*(k)}(\Sigma)\|_r + \|S^{*(k/2)}(\Sigma)\|_r). \quad (24)$$

Note that

$$S^{*(k)}(\Sigma) = \sum_{l=1}^k \sum_{-1 \leq j \leq \lfloor p/k \rfloor} M_{jk+l}^{*(k)}(\Sigma).$$

We have

$$\left\| \sum_{-1 \leq j \leq \lfloor p/k \rfloor} M_{jk+l}^{*(k)}(\Sigma) \right\|_r = \max_{-1 \leq j \leq \lfloor p/k \rfloor} \|M_{jk+l}^{*(k)}(\Sigma)\|_r,$$

for  $l \in \{1, 2, \dots, k\}$ , since the sum of matrices is a block diagonal matrix. Thus, we get

$$\begin{aligned} \|S^{*(k)}(\Sigma)\|_r &\leq \sum_{l=1}^k \left\| \sum_{-1 \leq j \leq \lfloor p/k \rfloor} M_{jk+l}^{*(k)}(\Sigma) \right\|_r \\ &\leq k \max_{1 \leq l \leq k} \left\| \sum_{-1 \leq j \leq \lfloor p/k \rfloor} M_{jk+l}^{*(k)}(\Sigma) \right\|_r \\ &\leq k \max_{1-k \leq l \leq p} \|M_l^{*(k)}(\Sigma)\|_r, \\ &= k \max_{1 \leq l \leq p} \|M_l^{*(k)}(\Sigma)\|_r, \end{aligned} \quad (25)$$

and

$$\|S^{*(k/2)}(\Sigma)\|_r \leq (k/2) \max_{1 \leq l \leq p} \|M_l^{*(k/2)}(\Sigma)\|_r.$$

Since  $\|M_l^{*(k/2)}(\Sigma)\|_r \leq \|M_l^{*(k)}(\Sigma)\|_r$  for  $l \in \{1, 2, \dots, p\}$ , we have

$$\|S^{*(k/2)}(\Sigma)\|_r \leq (k/2) \max_{1 \leq l \leq p} \|M_l^{*(k)}(\Sigma)\|_r. \quad (26)$$

Collecting (24), (25) and (26), we get

$$\|T_k(\Sigma)\|_r \leq 3 \max_{1 \leq l \leq p} \|M_l^{*(k)}(\Sigma)\|_r.$$

□

**Lemma 5.2.** *Let  $k$  and  $r$  be positive integers, and  $\tau$  and  $M_0$  be positive real numbers with  $\tau \geq k - 1$ . Suppose  $\Sigma_0 \in \mathcal{C}_k$  and  $T \sim W_k(\Sigma_0, \tau)$ . If  $\lambda_{\max}(\Sigma_0) \leq M_0$ , then there exists some positive constant  $C$  depending only on  $M_0$  and  $r$  such that*

$$E(\|T/\tau - \Sigma_0\|_2^r) \leq C \frac{5^k}{\tau^{r/2}}.$$

*Proof.* Let  $\Omega_\tau^{(k)} = \Sigma_0^{-1/2} T \Sigma_0^{-1/2} / \tau$ . We have

$$E(\|T/\tau - \Sigma_0\|_2^r) \leq \|\Sigma_0\|_2^r E(\|\Omega_\tau^{(k)} - I_k\|_2^r).$$

Since  $\|\Sigma_0\|_2^r$  is bounded by  $M_0^r$ , it suffices to show the upper bound of  $E(\|\Omega_\tau^{(k)} - I_k\|_2^r)$ .

By a property of Wishart distribution, we have

$$\Omega_\tau^{(k)} = \Sigma_0^{-1/2} T \Sigma_0^{-1/2} / \tau \sim W_k(I_k / \tau, \tau),$$

and

$$\begin{aligned} E(\|\Omega_\tau^{(k)} - I_k\|^r) &\leq \int_0^1 x^{r-1} P(\|\Omega_\tau^{(k)} - I_k\| > x) dx + \int_1^\infty x^{r-1} P(\|\Omega_\tau^{(k)} - I_k\| > x) dx \\ &\leq 2 \times 5^k \left\{ \int_0^1 x^{r-1} \exp(-\tau x^2 / 2^7) dx + \int_1^\infty x^{r-1} \exp(-\tau x / 2^7) dx \right\}, \end{aligned}$$

where the last inequality is satisfied by Lemma 4.4 in Lee et al. (2020). Integration by substitution and the definition of Gamma function give the inequalities

$$\begin{aligned} \int_0^1 x^{r-1} \exp(-\tau x^2 / 2^7) dx &\leq \frac{2^{7r/2-1}}{\tau^{r/2}} \int_0^\infty t^{r/2-1} \exp(-t) dt \\ &= \frac{2^{7r/2-1}}{\tau^{r/2}} \Gamma(r/2) \\ \int_1^\infty x^{r-1} \exp(-\tau x / 2^7) dx &\leq \left(\frac{2^7}{\tau}\right)^r \int_0^\infty t^{r-1} \exp(-t) dt \\ &= \left(\frac{2^7}{\tau}\right)^r \Gamma(r). \end{aligned}$$



Thus,

$$E(\|\Omega_\tau^{(k)} - I_k\|^r) \leq C_1 \frac{5^k}{\tau^{r/2}},$$

for some positive constant  $C_1$  depending only on  $r$ .

□

Next, we prove Lemmas [A.1-A.5](#).

*Proof of Lemma [A.1](#).* By Theorem 2.3.4 of Golub and Van Loan (2013), we have

$$\|\Sigma_0^{-1} - B_k(\Sigma_0)^{-1}\|_1 \leq \frac{\|B_k(\Sigma_0)^{-1}\|_1^2 \|\Sigma_0 - B_k(\Sigma_0)\|_1}{1 - \|B_k(\Sigma_0)^{-1}\{\Sigma_0 - B_k(\Sigma_0)\}\|_1}, \quad (27)$$

when  $\|B_k(\Sigma_0)^{-1}\{\Sigma_0 - B_k(\Sigma_0)\}\|_1 < 1$ . This inequality condition holds for all sufficiently large  $k$ , since  $\|B_k(\Sigma_0)^{-1}\|_1$  is bounded above by a constant and  $\|\Sigma_0 - B_k(\Sigma_0)\|_1 \leq Mk^{-\alpha}$ .

We show the boundedness of  $\|B_k(\Sigma_0)^{-1}\|_1$  below. Note that  $B_k(\Sigma_0) \in \mathcal{C}_p$  for all sufficiently large  $k$  since  $\lambda_{\min}\{B_k(\Sigma_0)\} \geq \lambda_{\min}(\Sigma_0) - \|B_k(\Sigma_0) - \Sigma_0\|$  (Lee et al., 2020, Lemma 4.14).

Thus, Theorem 2.4 of Demko et al. (1984) gives

$$\begin{aligned} \|B_k(\Sigma_0)^{-1}\|_1 &\leq \max_j \sum_{i=1}^p |w_{ij}| \\ &\leq C_1 \sup_j \sum_{i=1}^p (q_1^{2/k})^{|i-j|} \\ &\leq \frac{2C_1}{1 - q_1^{2/k}}, \end{aligned} \quad (28)$$

where  $B_k(\Sigma_0) = (w_{ij})$ ,  $C_1 = \{\|B_k(\Sigma_0)^{-1}\| \vee (1 + \kappa_1^{1/2})^2\} / (2\|B_k(\Sigma_0)\|)$ ,  $q_1 = (\kappa_1^{1/2} - 1) / (\kappa_1^{1/2} + 1)$  and  $\kappa_1$  is the spectral condition number of  $B_k(\Sigma_0)$ . To show that (28) is bounded, it suffices to show that  $\|B_k(\Sigma_0)^{-1}\|_2$  is bounded. By Lemma 4.14 in Lee et al. (2020), we have

$$\begin{aligned} \|B_k(\Sigma_0)^{-1}\|_2 &= \lambda_{\min}\{B_k(\Sigma_0)\}^{-1} \\ &\leq \frac{1}{\lambda_{\min}(\Sigma_0) - \|B_k(\Sigma_0) - \Sigma_0\|} \\ &\leq \frac{1}{\lambda_{\min}(\Sigma_0) - Mk^{-\alpha}}, \end{aligned} \quad (29)$$

which is bounded for all sufficiently large  $k$ . Thus, for all sufficiently large  $k$ ,  $\|B_k(\Sigma_0)^{-1}\{\Sigma_0 - B_k(\Sigma_0)\}\|_1 < 1$  and the inequality (27) is satisfied. By combining (27) and (28), we have that there exists some positive constant  $C_2$  depending only on  $M$ ,  $M_0$  and  $M_1$  such that

$$\begin{aligned} \|\Sigma_0^{-1} - B_k(\Sigma_0)^{-1}\|_1 &\leq \left(\frac{2C_1}{1 - q_1^{2/k}}\right)^2 \frac{Mk^{-\alpha}}{1 - 2C_1Mk^{-\alpha}/(1 - q_1^{2/k})} \\ &\leq C_2Mk^{-\alpha}, \end{aligned}$$

for all sufficiently large  $k$ .

Next, we consider the upper bound of  $\|\Sigma_0^{-1} - T_k(\Sigma_0)^{-1}\|_1$ . Note that  $T_k(\Sigma_0)$  is a  $k$ -band matrix and

$$\begin{aligned} \|T_k(\Sigma_0) - \Sigma_0\|_1 &\leq \|B_{\lfloor k/2 \rfloor}(\Sigma_0) - \Sigma_0\|_1 \\ &\leq M(\lfloor k/2 \rfloor)^{-\alpha}. \end{aligned} \tag{30}$$

In the same way as deriving the inequalities (28) and (29), we have

$$\begin{aligned} \|T_k(\Sigma_0)^{-1}\|_1 &\leq \frac{2C_3}{1 - q_2^{2/k}} \\ \|T_k(\Sigma_0)^{-1}\|_2 &\leq \frac{1}{\lambda_{\min}(\Sigma_0) - M(\lfloor k/2 \rfloor)^{-\alpha}}, \end{aligned} \tag{31}$$

where  $C_3 = \|T_k(\Sigma_0)^{-1}\| \vee (1 + \kappa_2^{1/2})^2 / (2\|T_k(\Sigma_0)\|)$ ,  $q_2 = (\kappa_2^{1/2} - 1) / (\kappa_2^{1/2} + 1)$  and  $\kappa_2$  is the spectral condition number of  $T_k(\Sigma_0)$ . Thus, we have  $\|T_k(\Sigma_0)^{-1}(\Sigma_0 - T_k(\Sigma_0))\|_1 < 1$  for all sufficiently large  $k$ , and apply Theorem 2.3.4 of Golub and Van Loan (2013). By Theorem 2.3.4 of Golub and Van Loan (2013), there exists some positive constant  $C_4$  depending only on  $M$ ,  $M_0$  and  $M_1$  such that

$$\begin{aligned} \|\Sigma_0^{-1} - T_k(\Sigma_0)^{-1}\|_1 &\leq \frac{\|T_k(\Sigma_0)^{-1}\|_1^2 \|\Sigma_0 - T_k(\Sigma_0)\|_1}{1 - \|T_k(\Sigma_0)^{-1}(\Sigma_0 - T_k(\Sigma_0))\|_1} \\ &\leq C_4(\lfloor k/2 \rfloor)^{-\alpha}, \end{aligned}$$

for all sufficiently large  $k$ . The last inequality holds by the inequalities (30) and (31).  $\square$

*Proof of Lemma A.2.* Two inequalities in Lemma 4.14 of Lee et al. (2020),

$$\begin{aligned} \lambda_{\min}\{T_k(S_n)\} &\geq \lambda_{\min}\{T_k(\Sigma_0)\} - \|T_k(S_n) - T_k(\Sigma_0)\| \\ \lambda_{\min}\{T_k(\Sigma_0)\} &\geq \lambda_{\min}(\Sigma_0) - \|\Sigma_0 - T_k(\Sigma_0)\|, \end{aligned}$$

imply

$$\begin{aligned} I[\lambda_{\min}\{T_k(S_n)\} \leq c] &\leq I\{\lambda_{\min}(\Sigma_0) - \|T_k(\Sigma_0) - \Sigma_0\| - \|T_k(S_n) - T_k(\Sigma_0)\| \leq c\} \\ &\leq I(\|T_k(S_n) - T_k(\Sigma_0)\| \geq c_k), \end{aligned} \quad (32)$$

where  $c_k = \lambda_{\min}(\Sigma_0) - M(\lfloor k/2 \rfloor)^{-\alpha} - c$ . The last inequality holds by the inequality (30). Since  $c \leq \lambda_{\min}(\Sigma_0)/2$  and  $\lfloor k/2 \rfloor > \{4M/\lambda_{\min}(\Sigma_0)\}^{1/\alpha}$ , we have  $c_k \geq \lambda_{\min}(\Sigma_0)/4$ . By Lemma 5.1, we have

$$\begin{aligned} P(\|T_k(S_n) - T_k(\Sigma_0)\| \geq c_k) &\leq P(\max_{1 \leq l \leq p} \|M_l^{(k)}(S_n - \Sigma_0)\| \geq c_k/3) \\ &\leq P(\|\Sigma_0\| \max_{1 \leq l \leq p} \|\Omega_{n,l}^{*(k)} - I_k\| \geq c_k/3) \\ &\leq P(M_0 \max_{1 \leq l \leq p} \|\Omega_{n,l}^{*(k)} - I_k\| \geq c_k/3) \\ &\leq p \max_{1 \leq l \leq p} P\{\|\Omega_{n,l}^{*(k)} - I_k\| \geq c_k/(3M_0)\}, \end{aligned}$$

where  $\Omega_{n,l}^{*(k)} = M_l^{(k)}(\Sigma_0)^{-1/2} M_l^{(k)}(S_n) M_l^{(k)}(\Sigma_0)^{-1/2}$  of which distribution is  $W_k(I_k/n, n)$ . Since  $c_k/(3M_0) < 1$ , Lemma 4.4 in Lee et al. (2020) gives

$$P\{\|\Omega_{n,l}^{*(k)} - I_k\| \geq c_k/(3M_0)\} \leq 2 \times 5^k \exp[-n\{c_k/(3M_0)\}^2/2^7]$$

Thus, combining this inequality with (32), we get

$$\begin{aligned} E(I[\lambda_{\min}\{T_k(S_n)\} \leq c]) &\leq E\{I(\|T_k(S_n) - T_k(\Sigma_0)\| \geq c_k)\} \\ &\leq p \max_{1 \leq l \leq p} P\{\|\Omega_{n,l}^{*(k)} - I_k\| \geq c_k/(3M_0)\} \\ &\leq 2p5^k \exp(-\lambda n), \end{aligned}$$

for some positive constant  $\lambda$  depending only on  $M_0$  and  $M_1$ .

□

*Proof of Lemma A.3.* Note, by Lemmas 5.1 and 2.1,

$$\begin{aligned} E(\|T_k^{(\epsilon_n)}(S_n) - \Sigma_0\|^4) &\leq 2^7 E(\|T_k(S_n) - \Sigma_0\|^4) + 4^3 \epsilon_n^4 \\ &\leq 2^{10} E(\|T_k(S_n) - T_k(\Sigma_0)\|^4) + 2^{10} \|\Sigma_0 - T_k(\Sigma_0)\|^4 + 4^3 \epsilon_n^4 \\ &\leq 2^{10} 3^4 E(\max_{1 \leq l \leq p} \|M_l^{(k)}(S_n - \Sigma_0)\|^4) + 2^{10} \|\Sigma_0 - T_k(\Sigma_0)\|^4 + 4^3 \epsilon_n^4. \end{aligned}$$

It suffices to show  $E(\max_{1 \leq l \leq p} \|M_l^{(k)}(S_n - \Sigma_0)\|^4)$  is bounded above. There exist some positive constants  $\rho_1$  and  $C_1$  depending only on  $M_0$  such that

$$\begin{aligned}
& E(\max_{1 \leq l \leq p} \|M_l^{(k)}(S_n - \Sigma_0)\|^4) \\
& \leq x^4 + E\{\max_{1 \leq l \leq p} \|M_l^{(k)}(S_n - \Sigma_0)\|^4 I(\max_{1 \leq l \leq p} \|M_l^{(k)}(S_n - \Sigma_0)\| > x)\} \\
& \leq x^4 + p^{1/2} \max_{1 \leq l \leq p} E(\|M_l^{(k)}(S_n - \Sigma_0)\|^8)^{1/2} P(\max_{1 \leq l \leq p} \|M_l^{(k)}(S_n - \Sigma_0)\| > x)^{1/2} \\
& \leq x^4 + C_1 p^{1/2} \frac{5^{k/2}}{n^2} \{2p5^k \exp(-nx^2 \rho_1)\}^{1/2},
\end{aligned}$$

for all  $0 < x < \rho_1$ . The last inequality is satisfied by Lemma 5.2 and Lemma 3 of Cai and Zhou (2010). We set  $x = \{2(\log p + k) \log 5 / (n\rho_1)\}^{1/2}$ , which can be smaller than an arbitrary positive constant for all sufficiently large  $n$ . Then, we have

$$\begin{aligned}
E(\max_{1 \leq l \leq p} \|M_l^{(k)}(S_n - \Sigma_0)\|^4) & \leq \left\{ \frac{2(\log p + k) \log 5}{n\rho_1} \right\}^2 + \frac{\sqrt{2}C_1 p 5^k}{n^2} \exp\{-(\log p + k) \log 5\} \\
& = \left\{ \frac{2(\log p + k) \log 5}{n\rho_1} \right\}^2 + \frac{\sqrt{2}C_1}{n^2} \exp(-(\log 5 - 1) \log p),
\end{aligned}$$

which is bounded by some positive constant depending only on  $M_0$  for all sufficiently large  $n$ .

□

*Proof of Lemma A.4.* Let  $c = \lambda_{\min}(\Sigma_0)/2$ . Since  $\lambda_{\min}\{T_k^{(\epsilon_n)}(S_n)_{11}\} \geq \lambda_{\min}\{T_k^{(\epsilon_n)}(S_n)\} \geq \epsilon_n$ , we have

$$\begin{aligned}
& E(\|T_k^{(\epsilon_n)}(S_n)_{11}^{-1} - \Sigma_{0,11}^{-1}\|^2) \\
& \leq \|\Sigma_{0,11}^{-1}\|^2 E(\|T_k^{(\epsilon_n)}(S_n)_{11}^{-1}\|^2 \|T_k^{(\epsilon_n)}(S_n)_{11} - \Sigma_{0,11}\|^2) \\
& \leq \frac{\|\Sigma_{0,11}^{-1}\|^2}{\epsilon_n^2} E(\|T_k^{(\epsilon_n)}(S_n)_{11} - \Sigma_{0,11}\|^2 I[\lambda_{\min}\{T_k(S_n)\} \leq c]) \tag{33}
\end{aligned}$$

$$+ \frac{\|\Sigma_{0,11}^{-1}\|^2}{c^2} E(\|T_k^{(\epsilon_n)}(S_n)_{11} - \Sigma_{0,11}\|^2). \tag{34}$$

By Lemmas A.2 and A.3, there exist some positive constants  $C_1$  and  $\lambda_1$  depending only on  $M_0$  and  $M_1$  such that

$$\begin{aligned}
(33) & \leq \frac{1}{M_1^2 \epsilon_n^2} E(\|T_k^{(\epsilon_n)}(S_n)_{11} - \Sigma_{0,11}\|^4)^{1/2} P[\lambda_{\min}\{T_k(S_n)\} \leq c]^{1/2} \\
& \leq \frac{C_1}{M_1^2 \epsilon_n^2} p^{1/2} 5^{k/2} \exp(-\lambda_1 n), \tag{35}
\end{aligned}$$

for all sufficiently large  $n$ . We also have

$$\begin{aligned}
(34) \quad &\leq \frac{1}{M_1^2 c^2} E(\|T_k^{(\epsilon_n)}(S_n) - \Sigma_0\|^2) \\
&\leq \frac{2^3}{M_1^2 c^2} E(\|T_k(S_n) - \Sigma_0\|^2) + \frac{4}{M_1^2 c^2} \epsilon_n^2 \\
&\leq C_2 \left\{ \frac{k + \log p}{n} + k^{-2\alpha} + \epsilon_n^2 \right\},
\end{aligned} \tag{36}$$

for some positive constant  $C_2$  depending only on  $M$ ,  $M_0$ ,  $M_1$  and  $\alpha$ . The second and last inequalities hold by Lemma 2.1 and Theorem 2 of Cai and Zhou (2010), respectively. Collecting (35) and (36), we complete the proof.  $\square$

*Proof of Lemma A.5.* Let  $c = \|\Sigma^{-1}\|_2 \wedge \|\Sigma'^{-1}\|_2$  and  $D = \Sigma' - \Sigma$ . Without loss of generality we suppose  $\|\Sigma^{-1}\|_2 = c$ . The Pinsker inequality gives

$$\begin{aligned}
\|P_\Sigma - P_{\Sigma'}\|_1^2 &\leq 2KL(P_{\Sigma'} \mid P_\Sigma) \\
&= n\{tr(\Sigma'\Sigma^{-1}) - \log \det(\Sigma'\Sigma^{-1}) - p\}, \\
&= n\{tr(D\Sigma^{-1}) - \log \det(I_p + D\Sigma^{-1})\},
\end{aligned} \tag{37}$$

where  $KL(\cdot \mid \cdot)$  is the Kullback-Leibler divergence. Before showing the upper bound of (37), we show

$$\log(1+x) \geq x - x^2, \text{ for } x > -1/2. \tag{38}$$

Let  $g(x) = \log(1+x) - x + x^2$ . Note

$$\begin{aligned}
g(0) &= 0 \\
g'(x) &< 0, \text{ if } -1/2 < x < 0 \\
g'(x) &> 0, \text{ if } x > 0,
\end{aligned}$$

where  $g'(x)$  is the derivative of  $g(x)$ . Thus, inequality (38) holds.

Now we give the upper bound of (37). Note that  $D\Sigma^{-1}$  is a similar matrix of  $\Sigma^{-1/2}D\Sigma^{-1/2}$  and the set of eigenvalues of  $D\Sigma^{-1}$  coincides with that of  $\Sigma^{-1/2}D\Sigma^{-1/2}$ . Let  $\{\lambda_1, \lambda_2, \dots, \lambda_p\}$

be the set of eigenvalues of  $D\Sigma^{-1}$ . If  $\lambda_i > -1/2$  for all  $i \in \{1, \dots, p\}$ , then inequality (38) gives

$$\begin{aligned}
-\log \det(I_p + D\Sigma^{-1}) &= -\sum_{i=1}^p \log(1 + \lambda_i) \\
&\leq -\sum_{i=1}^p \lambda_i + \sum_{i=1}^p \lambda_i^2 \\
&= -\text{tr}(D\Sigma^{-1}) + \sum_{i=1}^p \lambda_i^2.
\end{aligned}$$

By applying this inequality to (37), we have

$$\|P_\Sigma - P_{\Sigma'}\|_1^2 \leq n \sum_{i=1}^p \lambda_i^2.$$

It suffices to show  $\max_{i=1, \dots, p} |\lambda_i| < 1/2$  and  $\sum_{i=1}^p \lambda_i^2 \leq c^2 \|D\|_F^2$ . Since  $\|D\|_2 < 1/(2c)$ ,

$$\begin{aligned}
\max_{i=1, \dots, p} |\lambda_i| &\leq \|\Sigma^{-1/2} D \Sigma^{-1/2}\|_2 \\
&\leq \|D\|_2 \|\Sigma^{-1}\|_2 \\
&< 1/2.
\end{aligned}$$

Next, we show the upper bound of  $\sum_{i=1}^p \lambda_i^2$ . we have  $\Sigma^{-1} = UVU^T$  for some orthogonal matrix  $U$  and some diagonal matrix  $V$ , and

$$\begin{aligned}
\sum_{i=1}^p \lambda_i^2 &= \|\Sigma^{-1/2} D \Sigma^{-1/2}\|_F^2 \\
&= \|VU^T DUV\|_F^2 \\
&\leq \|V\|^2 \|U^T D U\|_F^2 \\
&= \|\Sigma^{-1}\|^2 \|D\|_F^2.
\end{aligned}$$

The second and third equalities hold since  $U$  is an orthogonal matrix. The first inequality holds since  $V$  is a diagonal matrix.

□

## 6 Proofs of Lemmas in Section S4

In this section, we prove Lemmas 4.1-4.4 which are presented in Section 4. For these proofs we present Lemmas 6.1 and 6.2.

**Lemma 6.1.** *Let  $n$ ,  $k$  and  $r$  be positive integers and  $M_0$  be a positive real number. Suppose  $\Sigma_0 \in \mathcal{C}_k$  and let the prior distribution  $\pi$  on  $\mathcal{C}_k$  be  $IW(A_n, \tau_n)$  for  $A_n \in \mathcal{C}_k$  and  $\tau_n > 2k$ . If  $(\tau_n - 2k) \vee \|A_n\| \vee k = o(n)$  and  $\|\Sigma_0\| \leq M_0$ , then there exists some positive constant  $C$  depending only on  $M_0$  and  $r$  such that*

$$E_{\Sigma_0}\{E^\pi(\|\Sigma - \Sigma_0\|^r \mid \mathbb{Z}_n)\} \leq Ck^r \frac{5^{3k/2}}{n^{r/2}},$$

for all sufficiently large  $n$ .

*Proof.* Let  $\hat{\Sigma} = (nS_n + A_n)/(n + \tau_n - k - 1)$ . We have

$$E_{\Sigma_0}\{E^\pi(\|\Sigma - \Sigma_0\|^r \mid \mathbb{Z}_n)\} \leq 2^{r-1}E_{\Sigma_0}\{E^\pi(\|\Sigma - \hat{\Sigma}\|^r \mid \mathbb{Z}_n)\} \quad (39)$$

$$+ 2^{r-1}E_{\Sigma_0}(\|\hat{\Sigma} - \Sigma_0\|^r). \quad (40)$$

For the upper bound of (40), we have

$$E_{\Sigma_0}(\|\hat{\Sigma} - \Sigma_0\|^r) \leq 2^{r-1}E_{\Sigma_0}\left(\left\|\frac{n}{n + \tau_n - k - 1}(S_n - \Sigma_0)\right\|^r\right) + 2^{r-1}\left\|\frac{A_n - (\tau_n - k - 1)\Sigma_0}{n + \tau_n - k - 1}\right\|^r.$$

Since  $(\tau_n - k - 1)/n = O(k/n)$  and  $\|A_n\| = o(n)$ , there exists some positive constant  $C_1$  depending only on  $M_0$  and  $r$  such that

$$\left\|\frac{A_n - (\tau_n - k - 1)\Sigma_0}{n + \tau_n - k - 1}\right\|^r \leq C_1\left(\frac{k}{n}\right)^r,$$

for all sufficiently large  $n$ . Lemma 5.2 gives

$$E_{\Sigma_0}\left(\left\|\frac{n}{n + \tau_n - k - 1}(S_n - \Sigma_0)\right\|^r\right) \leq C_2 \frac{5^k}{n^{r/2}},$$

for some positive constant  $C_2$  depending only on  $M_0$  and  $r$ . Thus, we have

$$(40) \leq 4^{r-1}C_1\left(\frac{k}{n}\right)^r + 4^{r-1}C_2 \frac{5^k}{n^{r/2}}. \quad (41)$$

Next, we show the upper bound of (39). We have

$$\begin{aligned}
& E_{\Sigma_0}\{E^\pi(\|\Sigma - \hat{\Sigma}\|^r \mid \mathbb{Z}_n)\} \\
&= E_{\Sigma_0}\{E^\pi(\|\hat{\Sigma}^{1/2}(\Omega_{n^*}^{(k)})^{-1}(I_k - \Omega_{n^*}^{(k)})\hat{\Sigma}^{1/2}\|^r \mid \mathbb{Z}_n)\} \\
&\leq E_{\Sigma_0}\{\|\hat{\Sigma}\|^r E^\pi(\|(\Omega_{n^*}^{(k)})^{-1}\|^r \|I_k - \Omega_{n^*}^{(k)}\|^r \mid \mathbb{Z}_n)\} \\
&\leq E_{\Sigma_0}\{\|\hat{\Sigma}\|^r E^\pi(\|(\Omega_{n^*}^{(k)})^{-1}\|^{2r} \mid \mathbb{Z}_n)^{1/2} E^\pi(\|I_k - \Omega_{n^*}^{(k)}\|^{2r} \mid \mathbb{Z}_n)^{1/2}\}, \tag{42}
\end{aligned}$$

where  $\Omega_{n^*}^{(k)} = \hat{\Sigma}^{1/2}\Sigma^{-1}\hat{\Sigma}^{1/2}$ . Note that  $[\Sigma \mid \mathbb{Z}_n] \sim IW_k(A_n + nS_n, n + \tau_n)$ . Since  $[\Sigma^{-1} \mid \mathbb{Z}_n] \sim W_k\{(A_n + nS_n)^{-1}, n + \tau_n - k - 1\}$  (Press, 2012), we have  $(n + \tau_n - k - 1)\Omega_{n^*}^{(k)} \sim W_k(I_k, n + \tau_n - k - 1)$ . Lemma 5.2 gives

$$\begin{aligned}
E^\pi(\|I_k - \Omega_{n^*}^{(k)}\|^{2r} \mid S_n)^{1/2} &\leq C_3 \frac{5^{k/2}}{(n + \tau_n - k - 1)^{r/2}} \\
&\leq C_3 \frac{5^{k/2}}{n^{r/2}}, \tag{43}
\end{aligned}$$

for some positive constant  $C_3$  depending only on  $M_0$  and  $r$ . Since  $[(\Omega_{n^*}^{(k)})^{-1} \mid \mathbb{Z}_n] \sim IW_k\{(n + \tau_n - k - 1)I_k, n + \tau_n\}$ , we have

$$\begin{aligned}
E^\pi(\|(\Omega_{n^*}^{(k)})^{-1}\|^{2r} \mid \mathbb{Z}_n) &\leq E^\pi\left(\left[\sum_{i=1}^k \{(\Omega_{n^*}^{(k)})^{-1}\}_{ii}\right]^{2r} \mid \mathbb{Z}_n\right) \\
&\leq k^{2r-1} \sum_{i=1}^k E^\pi[\{(\Omega_{n^*}^{(k)})^{-1}\}_{ii}^{2r} \mid \mathbb{Z}_n] \\
&\leq k^{2r} (n + \tau_n - k - 1)^{2r} \frac{1}{2^{2r}} \frac{\Gamma\{(n + \tau_n - 2k)/2 - 2r\}}{\Gamma\{(n + \tau_n - 2k)/2\}} \\
&= k^{2r} (n + \tau_n - k - 1)^{2r} \frac{1}{2^{2r}} \prod_{i=1}^{2r} \{(n + \tau_n - 2k)/2 - i\}^{-1} \\
&\leq \left(\frac{k}{2}\right)^{2r} \left\{ \frac{n + \tau_n - k - 1}{(n + \tau_n - 2k)/2 - 2r} \right\}^{2r}, \tag{44}
\end{aligned}$$

where  $\{(\Omega_{n^*}^{(k)})^{-1}\}_{ii}$  is the  $i$ th diagonal element of  $(\Omega_{n^*}^{(k)})^{-1}$ . The third inequality holds by Lemma 4.9 of Lee et al. (2020). By collecting (42), (43) and (44), we have that there exists some positive constant  $C_4$  depending only on  $M_0$  and  $r$  such that

$$(39) \leq C_4 k^r \frac{5^{k/2}}{n^{r/2}} E_{\Sigma_0}(\|\hat{\Sigma}\|^r), \tag{45}$$



for all sufficiently large  $n$ .

For the upper bound of  $E_{\Sigma_0}(\|\hat{\Sigma}\|^r)$ , there exist some positive constants  $C_5$  and  $C_6$  depending only on  $M_0$  and  $r$  such that

$$\begin{aligned}
E_{\Sigma_0}(\|\hat{\Sigma}\|^r) &\leq 2^{r-1}E_{\Sigma_0}(\|S_n\|^r) + \frac{2^{r-1}}{n^r}\|A_n\|^r \\
&\leq 4^{r-1}E_{\Sigma_0}(\|S_n - \Sigma_0\|^r) + 4^{r-1}\|\Sigma_0\|^r + \frac{2^{r-1}}{n^r}\|A_n\|^r \\
&\leq C_5 + C_6 \frac{5^k}{n^{r/2}},
\end{aligned} \tag{46}$$

for all sufficiently large  $n$ . The last inequality holds by Lemma 5.2. Collecting (45) and (46), we have

$$(39) \leq C_7 k^r \left( \frac{5^{k/2}}{n^{r/2}} + \frac{5^{3k/2}}{n^r} \right),$$

for some positive constant  $C_7$  depending only on  $M_0$  and  $r$ . Combining this inequality with (41), we complete the proof. □

**Lemma 6.2.** *Suppose the same setting of Lemma 6.1. If  $(\tau_n - 2k) \vee \|A_n\| \vee k = o(n)$ ,  $\|\Sigma_0\| \leq M_0$  and  $x < 4\|\Sigma_0\|$ , then there exist some positive constants  $C$  and  $\lambda$  depending only on  $M_0$  such that*

$$E_{\Sigma_0}\{P^\pi(\|\Sigma - \Sigma_0\| > x \mid \mathbb{Z}_n)\} \leq C5^k\{\exp(-\lambda nx^2) + \exp(-\lambda n)\},$$

for all sufficiently large  $n$ .

*Proof.* Let  $\hat{\Sigma} = (nS_n + A_n)/(n + \tau_n - k - 1)$ . We have

$$E_{\Sigma_0}\{P^\pi(\|\Sigma - \Sigma_0\| > x \mid \mathbb{Z}_n)\} \leq E_{\Sigma_0}\{P^\pi(\|\Sigma - \hat{\Sigma}\| > x/2 \mid \mathbb{Z}_n)\} + P_{\Sigma_0}(\|\hat{\Sigma} - \Sigma_0\| > x/2).$$

The upper bound of  $P_{\Sigma_0}(\|\hat{\Sigma} - \Sigma_0\| > x/2)$  is given as

$$\begin{aligned}
& P_{\Sigma_0}(\|\hat{\Sigma} - \Sigma_0\| > x/2) \\
&= P\left(\left\|\frac{n}{n + \tau_n - k - 1}(S_n - \Sigma_0) + \frac{A_n - (\tau_n - k - 1)\Sigma_0}{n + \tau_n - k - 1}\right\| > x/2\right) \\
&\leq P(\|S_n - \Sigma_0\| > x/4) + I\left(\|A_n\|/n + \frac{\tau_n - k - 1}{n + \tau_n - k - 1}\|\Sigma_0\| > x/4\right) \\
&\leq P(\|\Sigma_0\| \|\Omega_n^{(k)} - I_k\| > x/4) + I\left(\|A_n\|/n + \frac{\tau_n - k - 1}{n + \tau_n - k - 1}\|\Sigma_0\| > x/4\right) \\
&= P\{\|\Omega_n^{(k)} - I_k\| > x/(4\|\Sigma_0\|)\} + I\left(\|A_n\|/n + \frac{\tau_n - k - 1}{n + \tau_n - k - 1}\|\Sigma_0\| > x/4\right),
\end{aligned}$$

where  $\Omega_n^{(k)} = \Sigma_0^{-1/2} S_n \Sigma_0^{-1/2}$ , of which distribution is  $W_k(I_k/n, n)$ . Since  $\|A_n\| = o(n)$  and  $(\tau_n - k - 1)/(n + \tau_n - k - 1) = o(1)$ , we have

$$I\left(\|A_n\|/n + \frac{\tau_n - k - 1}{n + \tau_n - k - 1}\|\Sigma_0\| > x/4\right) = 0,$$

for all sufficiently large  $n$ . Since  $x < 4\|\Sigma_0\|$ , Lemma 4.4 in Lee et al. (2020) gives

$$P\{\|\Omega_n^{(k)} - I_k\| > x/(4\|\Sigma_0\|)\} \leq 2 \times 5^k \exp\{-nx^2/(2^{11}\|\Sigma_0\|^2)\}.$$

Thus, we have

$$P_{\Sigma_0}(\|\hat{\Sigma} - \Sigma_0\| > x/2) \leq 2 \times 5^k \exp\{-nx^2/(2^{11}\|\Sigma_0\|^2)\}, \quad (47)$$

for all sufficiently large  $n$ .

Next, we show the upper bound of  $E_{\Sigma_0}\{P^\pi(\|\Sigma - \hat{\Sigma}\| > x \mid \mathbb{Z}_n)\}$ . For arbitrary positive constants  $R_1$  and  $R_2$ , we have

$$\begin{aligned}
& E_{\Sigma_0}\{P^\pi(\|\Sigma - \hat{\Sigma}\| > x/2 \mid \mathbb{Z}_n)\} \\
&= E\{P^\pi(\|\hat{\Sigma}^{1/2}(\Omega_{n^*}^{(k)})^{-1}(I_k - \Omega_{n^*}^{(k)})\hat{\Sigma}^{1/2}\| > x/2 \mid \mathbb{Z}_n)\} \\
&\leq E\{P^\pi(\|\hat{\Sigma}\| \|(\Omega_{n^*}^{(k)})^{-1}\| \|I_k - \Omega_{n^*}^{(k)}\| > x \mid \mathbb{Z}_n)\} \\
&\leq E\{P^\pi(R_1\|(\Omega_{n^*}^{(k)})^{-1}\| \|I_k - \Omega_{n^*}^{(k)}\| > x \mid \mathbb{Z}_n)\} + P(\|\hat{\Sigma}\| > R_1) \\
&\leq E\{P^\pi(R_1 R_2 \|I_k - \Omega_{n^*}^{(k)}\| > x \mid \mathbb{Z}_n)\} + E[P^\pi\{\lambda_{\min}(\Omega_{n^*}^{(k)}) < R_2^{-1} \mid \mathbb{Z}_n\}] \\
&\quad + P(\|\hat{\Sigma}\| > R_1),
\end{aligned} \quad (48)$$

where  $\Omega_{n^*}^{(k)} = \hat{\Sigma}^{1/2} \Sigma^{-1} \hat{\Sigma}^{1/2}$ , of which distribution is  $W_k(I_k/(n + \tau_n - k - 1), n + \tau_n - k - 1)$ . If we set  $R_2^{-1} \leq [1 - \{k/(n + \tau_n - k - 1)\}^{1/2}]^2/4$ , Lemma 4.2 in Lee et al. (2020) gives that there exists some positive constant  $\lambda_1$  depending only on  $M_0$  and  $M_1$  such that

$$\begin{aligned} P^\pi\{\lambda_{\min}(\Omega_{n^*}^{(k)}) < R_2^{-1} \mid \mathbb{Z}_n\} &\leq 2 \exp\{-(n + \tau_n - k - 1)[1 - \{k/(n + \tau_n - k - 1)\}^{1/2}]^2/8\} \\ &\leq 2 \exp(-\lambda_1 n), \end{aligned} \quad (49)$$

for all sufficiently large  $n$ . If  $R_1 \in (||\Sigma_0||, 3||\Sigma_0||)$ , then

$$\begin{aligned} P(||\hat{\Sigma}|| > R_1) &\leq P(||\hat{\Sigma} - \Sigma_0|| > R_1 - ||\Sigma_0||) \\ &\leq 2 \times 5^k \exp\{-n(R_1 - ||\Sigma_0||)^2/(2^9 ||\Sigma_0||^2)\}, \end{aligned} \quad (50)$$

where the second inequality holds by (47). Since we can set  $R_2$  large enough to satisfy  $x/(R_1 R_2) < 1$ , Lemma 4.4 in Lee et al. (2020) gives

$$\begin{aligned} P^\pi(R_1 R_2 ||I_k - \Omega_{n^*}^{(k)}|| > x \mid \mathbb{Z}_n) &= P^\pi(||I_k - \Omega_{n^*}^{(k)}|| > x/(R_1 R_2) \mid \mathbb{Z}_n) \\ &\leq 2 \times 5^k \exp\left\{-\frac{(n + \tau_n - k - 1)x^2}{2^7 (R_1 R_2)^2}\right\}. \end{aligned} \quad (51)$$

By collecting the inequalities (48)-(51), we obtain that there exist some positive constants  $C_1$  and  $\lambda_2$  depending only on  $M_0$  and  $M_1$  such that

$$E_{\Sigma_0}\{P^\pi(||\Sigma - \hat{\Sigma}|| > x/2 \mid \mathbb{Z}_n)\} \leq C_1 5^k \{\exp(-\lambda_2 n x^2) + \exp(-\lambda_2 n)\},$$

for all sufficiently large  $n$ . Combining this inequality with (47), we complete the proof.  $\square$

Next, we prove the Lemmas 4.1-4.4.

*Proof of Lemma 4.1.* By Lemma 2.1 and 5.1, we have

$$\begin{aligned} &E_{\Sigma_0}\{E^{\pi^i}(|T_k^{(\epsilon_n)}(\Sigma) - \Sigma_0|^4 \mid \mathbb{Z}_n)\} \\ &\leq 2^7 E_{\Sigma_0}(E^{\pi^i}(|T_k(\Sigma) - \Sigma_0|^4 \mid \mathbb{Z}_n)) + 2^6 \epsilon_n^4 \\ &\leq 2^{10} E_{\Sigma_0}\{E^{\pi^i}(|T_k(\Sigma - \Sigma_0)|^4 \mid \mathbb{Z}_n)\} + 2^{10} ||T_k(\Sigma_0) - \Sigma_0||^4 + 2^6 \epsilon_n^4 \\ &\leq 2^{10} 3^4 E_{\Sigma_0}\{E^{\pi^i}(\max_{1 \leq i \leq p} ||M_i^{(k)}(\Sigma - \Sigma_0)||^4 \mid \mathbb{Z}_n)\} + 2^{10} \{M(\lfloor k/2 \rfloor)^{-\alpha}\}^4 + 2^6 \epsilon_n^4. \end{aligned} \quad (52)$$

Next, we have

$$\begin{aligned}
& E_{\Sigma_0}\{E^{\pi^i}(\max_{1 \leq i \leq p} \|M_i^{(k)}(\Sigma - \Sigma_0)\|^4 \mid \mathbb{Z}_n)\} \\
& \leq x^4 + E_{\Sigma_0}\{E^{\pi^i}(\max_{1 \leq i \leq p} \|M_i^{(k)}(\Sigma - \Sigma_0)\|^4 I(\max_{1 \leq i \leq p} \|M_i^{(k)}(\Sigma - \Sigma_0)\| > x) \mid \mathbb{Z}_n)\} \\
& \leq x^4 + E_{\Sigma_0}\{E^{\pi^i}(\max_{1 \leq i \leq p} \|M_i^{(k)}(\Sigma - \Sigma_0)\|^8 \mid \mathbb{Z}_n)\}^{1/2} E_{\Sigma_0}\{P^{\pi^i}(\max_{1 \leq i \leq p} \|M_i^{(k)}(\Sigma - \Sigma_0)\| > x \mid \mathbb{Z}_n)\}^{1/2} \\
& \leq x^4 + p \max_{1 \leq i \leq p} E_{\Sigma_0}\{E^{\pi^i}(\|M_i^{(k)}(\Sigma - \Sigma_0)\|^8 \mid \mathbb{Z}_n)\}^{1/2} \max_{1 \leq i \leq p} E_{\Sigma_0}\{P^{\pi^i}(\|M_i^{(k)}(\Sigma - \Sigma_0)\| > x \mid \mathbb{Z}_n)\}^{1/2}.
\end{aligned}$$

Note that  $M_l^{(k)}(\Sigma_0) \in \mathcal{F}_{k,\alpha}(M, M_0, M_1)$  and  $[M_l^{(k)}(\Sigma) \mid \mathbb{Z}_n] \sim IW_k(M_l^{(k)}(nS_n + A_n), n + \nu_n - 2p + 2k)$  (Press, 2012). If  $x < 4\|M_l^{(k)}(\Sigma_0)\|$ , then Lemmas 6.1 and 6.2 give that there exist some positive constants  $C_1$  and  $\lambda_1$  depending only on  $M_0$  and  $M_1$  such that

$$\begin{aligned}
& p \max_{1 \leq i \leq p} E_{\Sigma_0}\{E^{\pi^i}(\|M_i^{(k)}(\Sigma - \Sigma_0)\|^8 \mid \mathbb{Z}_n)\}^{1/2} \max_{1 \leq i \leq p} E_{\Sigma_0}\{P^{\pi^i}(\|M_i^{(k)}(\Sigma - \Sigma_0)\| > x \mid \mathbb{Z}_n)\}^{1/2} \\
& \leq C_1 p k^4 5^{5k/2} n^{-2} \{\exp(-\lambda_1 n x^2) + \exp(-\lambda_1 n)\}, \tag{53}
\end{aligned}$$

for all sufficiently large  $n$ . By setting  $x = 3 \log p / (\lambda_1 n)$ , which is smaller than an arbitrary positive constant for sufficiently large  $n$ , We show that (53) is bounded above by some positive constant for all sufficiently large  $n$ . Since  $\epsilon_n = O(1)$ , (52) is bounded by some positive constant depending only on  $M_0, M_1, M$  and  $\alpha$ .

□

*Proof of Lemma 4.2.* By inequality (32), we have

$$I[\lambda_{\min}\{T_k(\Sigma)\} \leq c] \leq I(\|T_k(\Sigma - \Sigma_0)\| \geq c_k)$$

where  $c_k = \lambda_{\min}(\Sigma_0) - M(\lfloor k/2 \rfloor)^{-\alpha} - c$ . Since  $c \leq \lambda_{\min}(\Sigma_0)/2$  and  $\lfloor k/2 \rfloor > \{4M/\lambda_{\min}(\Sigma_0)\}^{1/\alpha}$ , we have  $c_k \geq \lambda_{\min}(\Sigma_0)/4$ . There exist some positive constants  $C$  and  $\lambda$  depending only on  $M_0$  and  $M_1$  such that

$$\begin{aligned}
E_{\Sigma_0}(P^{\pi^i}[\lambda_{\min}\{T_k(\Sigma)\} \leq c \mid \mathbb{Z}_n]) & \leq E_{\Sigma_0}\{P^{\pi^i}(\lambda_{\min}(\|T_k(\Sigma - \Sigma_0)\| \geq c_k \mid \mathbb{Z}_n))\} \\
& \leq p \max_{1 \leq l \leq p} E_{\Sigma_0}\{P^{\pi^i}(\|M_l^{(k)}(\Sigma - \Sigma_0)\| \geq c_k/3 \mid \mathbb{Z}_n)\} \\
& \leq p C 5^k [\exp\{-\lambda n (c_k/3)^2\} + \exp(-\lambda n)],
\end{aligned}$$

for all sufficiently large  $n$ . The second inequality is satisfied by Lemma 5.1. For the third inequality, Lemma 6.2 is used. Note  $M_l^{(k)}(\Sigma_0) \in \mathcal{F}_{k,\alpha}(M, M_0, M_1)$ ,  $[M_l^{(k)}(\Sigma) \mid \mathbb{Z}_n] \sim IW_k\{M_l^{(k)}(nS_n + A_n), n + \nu_n - 2p + 2k\}$  and  $c_k/3$  satisfies

$$\begin{aligned} c_k/3 &\leq \lambda_{\min}(\Sigma_0) \\ &\leq \lambda_{\min}\{M_l^{(k)}(\Sigma_0)\} \\ &\leq 4\|M_l^{(k)}(\Sigma_0)\|, \end{aligned}$$

for all  $l \in \{1, 2, \dots, p\}$ . □

*Proof of Lemma 4.3.* By Lemmas 2.1 and 5.1, we have

$$\begin{aligned} &E_{\Sigma_0}\{E^{\pi^i}(\|\Sigma_0 - T_k^{(\epsilon_n)}(\Sigma)\|^2 \mid \mathbb{Z}_n)\} \\ &\leq 2^3 E_{\Sigma_0}\{E^{\pi^i}(\|\Sigma_0 - T_k(\Sigma)\|^2 \mid \mathbb{Z}_n)\} + 4\epsilon_n^2 \\ &\leq 2^4 E_{\Sigma_0}\{E^{\pi^i}(\|T_k(\Sigma_0) - T_k(\Sigma)\|^2 \mid \mathbb{Z}_n)\} + 2^4\|T_k(\Sigma_0) - \Sigma_0\|^2 + 4\epsilon_n^2 \\ &\leq 2^4 3^2 E_{\Sigma_0}\{E^{\pi^i}(\max_{1 \leq l \leq p} \|M_l^{(k)}(\Sigma_0 - \Sigma)\|^2 \mid \mathbb{Z}_n)\} + 2^4(M\lfloor k/2 \rfloor^{-\alpha})^2 + 4\epsilon_n^2. \end{aligned} \quad (54)$$

Note  $M_l^{(k)}(\Sigma_0) \in \mathcal{F}_{k,\alpha}(M, M_0, M_1)$ ,  $[M_l^{(k)}(\Sigma) \mid \mathbb{Z}_n] \sim IW_k\{M_l^{(k)}(nS_n + A_n), n + \nu_n - 2p + 2k\}$ . Thus, for an arbitrary positive real number  $x$  with  $x < 4 \min_{1 \leq l \leq p} \|M_l^{(k)}(\Sigma_0)\|$ , there exist some positive constants  $C_1$  and  $\lambda_1$  depending only on  $M_0$  such that

$$\begin{aligned} &E_{\Sigma_0}\{E^{\pi^i}(\max_{1 \leq l \leq p} \|M_l^{(k)}(\Sigma_0 - \Sigma)\|^2 \mid \mathbb{Z}_n)\} \\ &\leq x^2 + E_{\Sigma_0}[E^{\pi^i}\{\max_{1 \leq l \leq p} \|M_l^{(k)}(\Sigma_0 - \Sigma)\|^2 I(\max_{1 \leq l \leq p} \|M_l^{(k)}(\Sigma_0 - \Sigma)\| > x) \mid \mathbb{Z}_n\}] \\ &\leq x^2 + p \max_{1 \leq l \leq p} E_{\Sigma_0}\{E^{\pi^i}(\|M_l^{(k)}(\Sigma_0 - \Sigma)\|^4 \mid \mathbb{Z}_n)\}^{1/2} \max_{1 \leq l \leq p} E_{\Sigma_0}\{E^{\pi^i}(\|M_l^{(k)}(\Sigma_0 - \Sigma)\| > x \mid \mathbb{Z}_n)\}^{1/2} \\ &\leq x^2 + C_1 p k^2 \frac{5^3}{n} 5^k \{\exp(-\lambda_1 n x^2) + \exp(-\lambda_1 n)\}, \end{aligned}$$

for all sufficiently large  $n$ . The last inequality holds by Lemmas . By setting  $x^2 = 2(\log p + k \log 5)/n\lambda_1$ , which is lower than an arbitrary positive constant for all sufficiently large  $n$ , we have

$$E_{\Sigma_0}\{E^{\pi^i}(\max_{1 \leq l \leq p} \|M_l^{(k)}(\Sigma_0 - \Sigma)\|^2 \mid \mathbb{Z}_n)\} \leq C_2 \left( \frac{\log p + k}{n} \right),$$

for some positive constants  $C_2$  depending only on  $M_0$ . Combining this inequality with (54), we complete the proof.  $\square$

*Proof of Lemma 4.4.* Let  $c = \lambda_{\min}(\Sigma_0)/2$ . Since  $\lambda_{\min}\{T_k^{(\epsilon_n)}(\Sigma)_{11}\} \geq \lambda_{\min}\{T_k^{(\epsilon_n)}(\Sigma)\} \geq \epsilon_n$ , we have

$$\begin{aligned}
& E_{\Sigma_0}\{E^{\pi^i}(\|\Sigma_{0,11}^{-1} - T_k^{(\epsilon_n)}(\Sigma)_{11}^{-1}\|^2 \mid \mathbb{Z}_n)\} \\
& \leq \|\Sigma_0^{-1}\|^2 E_{\Sigma_0}\{E^{\pi^i}(\|T_k^{(\epsilon_n)}(\Sigma)_{11}^{-1}\|^2 \|\Sigma_{0,11} - T_k^{(\epsilon_n)}(\Sigma)_{11}\|^2 \mid \mathbb{Z}_n)\} \\
& \leq \frac{1}{M_1^2 c^2} E_{\Sigma_0}\{E^{\pi^i}(\|\Sigma_{0,11} - T_k^{(\epsilon_n)}(\Sigma)_{11}\|^2 \mid \mathbb{Z}_n)\} \\
& \quad + \frac{1}{M_1^2 \epsilon_n^2} E_{\Sigma_0}\{E^{\pi^i}(\|\Sigma_{0,11} - T_k^{(\epsilon_n)}(\Sigma)_{11}\|^2 I[\lambda_{\min}\{T_k(\Sigma)\} \leq c] \mid \mathbb{Z}_n)\} \\
& \leq \frac{1}{M_1^2 c^2} E_{\Sigma_0}\{E^{\pi^i}(\|\Sigma_{0,11} - T_k^{(\epsilon_n)}(\Sigma)_{11}\|^2 \mid \mathbb{Z}_n)\} \\
& \quad + \frac{1}{M_1^2 \epsilon_n^2} E_{\Sigma_0}\{E^{\pi^i}(\|\Sigma_{0,11} - T_k^{(\epsilon_n)}(\Sigma)_{11}\|^4 \mid \mathbb{Z}_n)\}^{1/2} E_{\Sigma_0}\{E^{\pi^i}(I[\lambda_{\min}\{T_k(\Sigma)\} \leq c] \mid \mathbb{Z}_n)\}^{1/2}
\end{aligned} \tag{55}$$

For the upper bound of (55), Lemma 4.3 gives

$$\begin{aligned}
E_{\Sigma_0}\{E^{\pi^i}(\|\Sigma_{0,11} - T_k^{(\epsilon_n)}(\Sigma)_{11}\|^2 \mid \mathbb{Z}_n)\} & \leq E_{\Sigma_0}\{E^{\pi^i}(\|\Sigma_0 - T_k^{(\epsilon_n)}(\Sigma)\|^2 \mid \mathbb{Z}_n)\} \\
& \leq C_1 \left( \frac{k + \log p}{n} + k^{-2\alpha} + \epsilon_n^2 \right),
\end{aligned}$$

for some positive constant  $C_1$  depending only on  $M$ ,  $M_0$ ,  $M_1$  and  $\alpha$ . Lemmas 4.1 and 4.2 gives that there exist positive constants  $C_2$  and  $\lambda$  depending only on  $M$ ,  $M_0$ ,  $M_1$  and  $\alpha$  such that

$$(56) \leq C_2 \frac{p^{1/2} 5^{k/2}}{\epsilon_n^2} \exp(-\lambda_1 n),$$

for all sufficiently large  $n$ . Collecting the upper bound of (55) and (56), we complete the proof.  $\square$

## References

P. J. Bickel and E. Levina. Regularized estimation of large covariance matrices. *The Annals of Statistics*, pages 199–227, 2008.

- T. T. Cai and H. H. Zhou. Optimal rates of convergence for covariance matrix estimation. *The Annals of Statistics*, 38(4):2118–2144, 2010.
- S. Demko, W. F. Moss, and P. W. Smith. Decay rates for inverses of band matrices. *Mathematics of computation*, 43(168):491–499, 1984.
- G. H. Golub and C. F. Van Loan. Matrix computations, 4th. *Johns Hopkins*, 2013.
- K. Lee, K. Lee, and J. Lee. Post-processed posteriors for banded covariances. *arXiv preprint arXiv:2011.12627*, 2020.
- S. J. Press. *Applied multivariate analysis: using Bayesian and frequentist methods of inference*. Courier Corporation, 2012.
